# Supplementary material for: Switch 2.0: A Modern Platform for Planning High-Renewable Power Systems
Source: arXiv:1804.05481 ancillary file (2018-10-17)
Supplement: Supplementary file 1 [file Supplementary.pdf]

# Switch 2.0: A Modern Platform for Planning High-Renewable Power Systems

Matthias Fripp[a], Josiah Johnston[a,b,c], Rodrigo Henríquez[d,e], and Benjamín Maluenda[d]

[a] Department of Electrical Engineering, University of Hawaii, Hawaii, USA.

[b] Energy and Resources Group, University of California, Berkeley, California, USA.

[c] Josiah Johnston, PhD Consulting & Research.

[d] Department of Electrical Engineering and Computer Sciences, University of California, Berkeley, USA.

[e] Department of Electrical Engineering, Pontificia Universidad Católica de Chile, Santiago, Chile.

Submitted to SoftwareX

**Supplementary Material**

# Contents


**1 Introduction** **3**

**2 Requirements for high-renewable planning** **3**

2.1 Temporal, spatial, and operational resolution . . . 3

2.1.1 Time resolution & sampling . . . 3

2.1.2 Spatial resolution . . . 4

2.1.3 Operational resolution . . . 4

2.2 Managing computational complexity . . . 5

2.3 Transparency and replicability . . . 5

**3 Switch installation and usage** **6**

3.1 Setup . . . 6

3.2 Usage . . . 6

3.3 Extensibility . . . 7

**4 Switch model formulation** **8**

4.1 Typographical conventions . . . 8

4.2 Overview . . . 9

4.2.1 Objective function . . . 9

4.2.2 Operational constraints . . . 10

4.2.2.1 Power balance . . . 10

4.2.2.2 Dispatch . . . 11

4.2.2.3 Minimum up and down times . . . 11

4.2.3 Investment constraints . . . 12

4.2.3.1 Power system construction . . . 12

4.2.3.2 Maximum investment . . . 12

4.3 Switch modules . . . 12

4.3.1 timescales . . . 12

4.3.2 financials . . . 14

4.3.3 balancing.load_zones . . . 15

4.3.4 energy_sources.properties . . . 16

4.3.5 generators.core.build . . . 16

4.3.6 generators.core.gen_discrete_build . . . 18

4.3.7 generators.core.dispatch . . . 18
4.3.8 energy_sources.fuel_costs.simple . . . 19
4.3.9 energy_sources.fuel_costs.markets . . . 19
4.3.10 transmission.transport.build . . . 20
4.3.11 transmission.transport.dispatch . . . 21
4.3.12 generators.core.no_commit . . . 22
4.3.13 generators.core.commit.operate . . . 23
4.3.14 generators.core.commit.discrete . . . 24
4.3.15 generators.core.commit.fuel_use . . . 24
4.3.16 transmission.local_td . . . 26
4.3.17 balancing.demand_response.simple . . . 27
4.3.18 generators.extensions.hydro_simple . . . 27
4.3.19 generators.extensions.hydro_system . . . 28
4.3.20 generators.extensions.storage . . . 30
4.3.21 policies.rps_simple . . . 31
4.3.22 policies.carbon_policies . . . 32
4.3.23 balancing.unserved_load . . . 32
4.3.24 balancing.planning_reserves . . . 33
4.3.25 balancing.operating_reserves.areas . . . 34
4.3.26 balancing.operating_reserves.spinning_reserves . . . 34
4.3.26.1 Unit-based contingency . . . 36
4.3.26.2 Project-based contingency . . . 37
4.3.26.3 Dynamic reserve constraints . . . 37
4.3.27 balancing.operating_reserves.spinning_reserves_advanced . . . 38

**5 References** **40**

# 1 Introduction

This document presents Supplementary Material for the paper submitted to SoftwareX.

The document is organized as follows. Section 2 describes requirements for modeling high-renewable electric power systems, and common approaches. Section 3 presents the installation and usage of Switch. Section 4 presents the complete formulation of Switch 2.0, presenting the key equations defining the model, and then describing the sets, variables and constraints that are defined in each module.

# 2 Requirements for high-renewable planning

## 2.1 Temporal, spatial, and operational resolution

### 2.1.1 Time resolution & sampling

Multiple timescales ranging from hours to decades need to be represented in capacity planning models for high-renewable grids.

Grid assets have typical lifetimes of decades, so accurate valuation requires modeling an evolving grid over corresponding timeframes, e.g. multi-stage investments. Models that focus on single-step, incremental change from today's power system risk yielding stranded assets or excessive system costs [1].

Operational timescales must reflect annual, seasonal, weekly, diurnal, and hourly variability of load and wind, solar, and hydro generation profiles. Historically, planning models could focus on the probability distribution for loads without regard to the chronological sequence of system conditions because hour-to-hour balancing requirements were easy to address outside of the planning process. However, the added variability of renewables means that hour-to-hour balancing considerations now have a significant impact on the planning problem [1–10].

Capacity planning models have generally used unordered sets of timepoints to describe load and renewable production profiles, also called "timeslice" or "load duration curve" methodologies [11–15]. Typically, timeslices are selected by stratified sampling of loads, creating a load duration curve, neglecting covariance with renewable timeseries. This methodology does not capture the chronological sequence of the underlying timeseries, although chronological constraints can be added separately [3, 16]. Chronological timeseries are commonly used in production cost models and are beginning to be integrated into capacity planning models [3, 16, 17]. While full timeseries of 8760 annual hours can be computationally tractable for production cost models, sampling techniques are generally required in capacity expansion models to manage computationally complexity [18].

Switch 1.0 introduced a hierarchical time structure, using multiple investment periods, each containing a collection of independent, day-long timeseries sampled from historical conditions in order to represent seasonal variations. This enabled modeling of renewable energy transitions, unit commitment and demand response in a number of case studies [19–25]. Switch 2.0 defines more flexible and general temporal data structures capable of describing timeslices, sampled timeseries of any duration, or extensive 8760 annual hourly timeseries. Each investment period contains one or more timeseries of arbitrary duration, resolution and weight. Each timeseries contains one or more

sequential timepoints of equal duration. The separation of duration (hours) and weight (frequency of occurrence in a year) is necessary to describe both thermodynamic and statistical properties of the sampled timeseries.

In addition, more states (for future costs, loads or weather) can be incorporated and solved in parallel via the Pyomo Stochastic Programming (PySP) component of the Pyomo optimization framework [26].

#### 2.1.2 Spatial resolution

Modern power systems are managed over large geographical scales, and power is carried over networks that have varying degrees of congestion at different locations. The behavior of renewable resources also varies between different locations. Consequently, capacity expansion models for renewable-dominated power systems must consider the spatial distribution of resources and loads and the ability of the network to move power between them [1, 27]. It is especially important to select a network formulation that is detailed enough for the planning task at hand, but not so complex that it becomes computationally intractable.

Existing models use several approaches to represent network capabilities. A basic strategy is to use a single-zone (*copperplate*) formulation, which ignores restrictions on spatial transfer of power [12, 28]. These are best suited for small, strong networks. Several capacity expansion models use a *transport model* to represent inter-regional power transfers [19, 29]. In a transport model, the study region is divided into zones which are internally well-connected but have constrained connections (flowgates) to neighboring zones. Power transfer through each flowgate is a decision variable. Transport models provide an attractive balance between granularity and tractability in expansion models, because they represent the capabilities of the network and the cost of expansion using only linear terms. A limited number of capacity expansion models use *DC network models* to represent the physical properties of the electrical network in greater detail [11, 30]. This formulation represents much of the network's physical behavior, but introduces numerous additional decision variables and constraints relative to simpler models. In particular, it is necessary to introduce either quadratic terms or "big-M" constraints with binary variables to represent expansion of the transmission network, significantly increasing solution times [11, 31]. Finally, *AC network models* are the "gold standard" for modeling the physical behavior of the network, but these are highly nonlinear, requiring iterative solutions. We are not aware of their use in any publicly available capacity expansion model.

Switch 2.0 has full support for copperplate and transport models. The modular architecture also allows use of other network models: an experimental module provides security-constrained AC power flow in a production-cost environment, and future work will add DC power flow, similar to the formulation in [31].

#### 2.1.3 Operational resolution

Capacity expansion planning models for high-renewable power systems must consider operating reserve requirements and unit commitment (UC) decisions, in order to analyze their impacts on investment decisions [32, 33]. Technologies such as storage, pumped hydro, hydro reservoirs, and demand response must also be included in these models, because they can provide significant low-

emission operational flexibility, potentially deferring investments of fossil-based generation capacity [34–36].

Traditionally, capacity expansion models have assumed that load could be met in every timepoint by any generator, ignoring UC and spinning reserve decisions [11, 27, 37]. However, consideration of UC and reserve requirements produces a better assessment of which technologies should be built and operated, especially in systems with high penetration of renewable sources [4, 16]. UC is usually assessed by solving MILP with binary variables to represent on/off decisions and constraints representing minimum up and down times, startup costs, etc. These binary variables and time-coupling constraints yield computationally expensive problems, but clustering may reduce solution times [5, 38].

Switch 1.0 modeled generator dispatch and a linear relaxation of the UC problem. Switch 2.0 offers both linearized UC and MILP UC via user-selectable modules. Users may also optionally provide detailed incremental heat rate curves, minimum up and down times, startup costs and other elements. Additional modules customizes dispatch and investment rules for individual technologies such as storage, hydroelectric generators, and demand response.

### 2.2 Managing computational complexity

The preceding sections describe a number of possible formulations for each of the major elements of the power system capacity expansion problem. It is not possible to include the most detailed formulation for every component in a practical capacity expansion model, because the number of constraints and variables becomes too large to solve in reasonable time. Instead, in order to balance accuracy and performance, practical capacity expansion models include more detail in areas that are of particular interest or strongly affect the outcome of the specific study, and less detail in other areas.

Almost all previous work has embedded decisions about operational detail directly in the mathematical formulation or computational implementation, making it difficult for other users to adapt those models to explore new questions. To address this challenge, Switch 2.0 takes a modular approach which allows the formulation to be easily customized around the needs of a new study. This modular architecture allows comparison of reduced-form formulations to determine which factors are relevant in a particular context, or to compare new formulations against established benchmarks using a single software platform and dataset. Users can also switch easily between distinct modeling modes, such as running a sparse capacity-expansion model, followed by a more detailed production-cost assessment of the proposed portfolio.

### 2.3 Transparency and replicability

The source code and data of energy models used by academia, industry, and public organizations have not typically been made publicly and freely available. The traditional planning methodology used by industry has been to manually construct investment plans (candidate portfolios) using expert knowledge and heuristics [39], which are typically assessed *ex-post* using commercial production cost models. This missing transparency has hindered scientific discussion on model quality and cross-validation of results, as well as being a barrier to stakeholder engagement [40, 41]. A

critical review of the assumptions, data, tools, and interpretations is necessary for providing scientifically sound contributions to political and public debates [1, 40, 42]. Integrated resource planning and open stakeholder engagement are gradually replacing opaque methods, and capacity expansion optimization models are increasingly used to guide selection of candidate portfolios [43–45].

The Switch platform implements best practices for scientific computing [46] that enable replicable analysis, development, review and collaboration by an open community, automated testing, and embedded documentation, enabling scientifically sound contributions to political and public debates [40, 42]. Platform architecture, software engineering features, and a permissive open-source license allow users to access and customize existing modules, or add new ones, to fit their specific needs while re-using core components. Thus, Switch 2.0 is a scalable analytical platform that can be used by a large and diverse community of researchers and industry, promote greater collaboration and communication between stakeholders, and aid in the dissemination of cutting-edge planning tools. Several examples are included in the Switch package to support its implementation in educational environments and ease the learning process.

# 3 Switch installation and usage

## 3.1 Setup

Prerequisites for using Switch are a Python 2.7 development environment and optimization software compatible with Pyomo. Switch is listed and available on the Python Package Index as `switch_model` and can be directly installed as a package with the `pip` command, as follows:

```
pip install switch_model
```

Users that seek to customize the source code and/or contribute with the public repository may install Switch by downloading or cloning the GitHub repository (`https://github.com/switch-model/switch`) into a local folder in their workstation and using the `pip` package manager to add it to the computer's Python installation by executing the following command in a terminal:

```
pip install --upgrade --editable .
```

Any missing Python package dependencies will be automatically installed in the process. The `pip` package manager may be used to maintain an updated version of Switch, though more frequent updates are available by using the Git software to pull most recent versions directly from the public repository.

Users can find instructions for installing external dependencies (e.g., numerical solvers) and pre-release versions of Switch at the model website at `http://www.switch-model.org`.

## 3.2 Usage

Switch is run from the operating system's command line environment. The `switch` command can be used to solve either single scenario instances or multiple scenarios in one run. Various options

may be specified either as command line arguments or in an options file. These options can be listed using the `--help` flag on the command line. The following command is an example for solving a single scenario model with default options and verbose console output:

```
switch solve --verbose
```

To solve a scenario, Switch first defines an *abstract model* based on the module list that the user has specified in `modules.txt`, creating the components needed to model the required features of the scenario. Next, each module in the list is provided an opportunity to read input data from disk that is collectively used to instantiate the abstract model into a *model instance* that represents a concrete scenario. This allows a high degree of flexibility in the definition of time scales, aggregation of projects, system topology, and other aspects. Inputs are read by Switch from a set of text files, which must be specified in one of the following formats.

- *.dat* files: These follow the AMPL .dat format and are used to specify simple key-value parameters.
- *.tab* files: These are tab-separated column files and are used to specify indexed parameters.

After the model is populated with inputs, the instance is used to generate an optimization problem in standard matrix form, which is passed to the solver along with any user-defined options for the optimization process, such as a specific solution method, optimality gap, or any other solver parameter. Once the solver software finishes, the Switch instance is populated with the results and outputs are exported. All variable values are saved by default in tab-separated value files for user examination. In addition, the user may add custom export modules to process results in any desired fashion and/or interactively explore the optimal instance in a Python console.

Figure 1 schematizes the usage of Switch. The set of examples contained in the repository may be examined for further specificity.

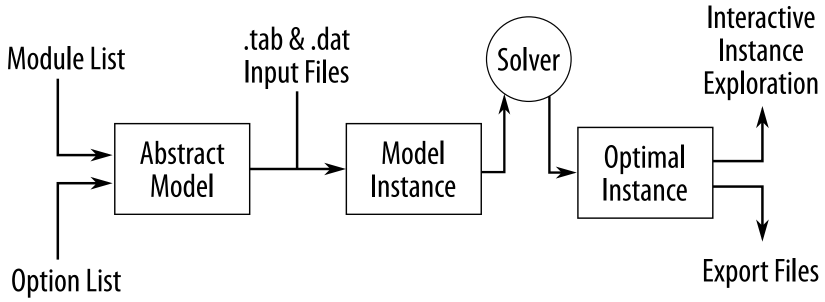


Figure 1: Conventional process of formulation and solving of single scenarios by Switch.

### 3.3 Extensibility

The modular structure of Switch enables a smooth integration of custom user code in the form of new modules or edition of existing ones. The following hooks are provided so that modules

can extend the capabilities of the model. A utility function iterates over the modules listed in `modules.txt` and calls each function in turn to construct an abstract model and instantiate it with particular inputs. All functions are optional and will be skipped if undefined by a given module.

- `define_dynamic_lists`: A module may construct special sets (defined as Python lists) to which other loaded modules may register components. Current use cases are energy injections and withdrawals at power balancing nodes, as well as cost components of the objective function. A new custom module would use these sets to register its impact on power balance of the grid, and to describe its investment and/or operational costs. Each element of these dynamic lists are some type of model component (parameters, variables or expressions) with standardized indexing rules and physical units to ensure compatibility with other expressions in a summation.
- `define_components`: Modules define sets, parameters, decision variables, expressions, and constraints in this function, as well as adding components to dynamic lists where appropriate.
- `define_dynamic_components`: This function may define additional components that require knowledge of other loaded modules. Usually creates variables and constraints based on components registered in dynamic lists.
- `load_inputs`: Modules load required and optional inputs into a Pyomo *DataPortal* in this function, based on a path to an inputs directory.
- `post_solve`: This function gets executed after the instance is solved, for post-processing and exporting results.

# 4 Switch model formulation

This section presents all of Switch's standard modules, detailing the sets, variables, parameters, and constraints that are defined in each module. It begins with some typgraphical conventins, then provides an overview of the key elements that form the core of the model, and finally gives complete details on all the modules included with Switch 2.0.

## 4.1 Typographical conventions

Figure 2 depicts the hierarchy of modules that are available in Switch. Python names for each module are written in lowercase with underscores instead of spaces and dots to identify branches in the package tree; e.g., Switch Model—Generators—Core—no commit is referenced in model code as `switch_model.generators.core.no_commit`.

In this document, we use the following typographical conventions regarding the names of model elements:

- Uppercase italic letters (e.g. $P, B, K$) define decision variables (values chosen by the model).
- Lowercase italic letters (e.g. $l, h, c$) define parameters (input data) and indexes over sets.

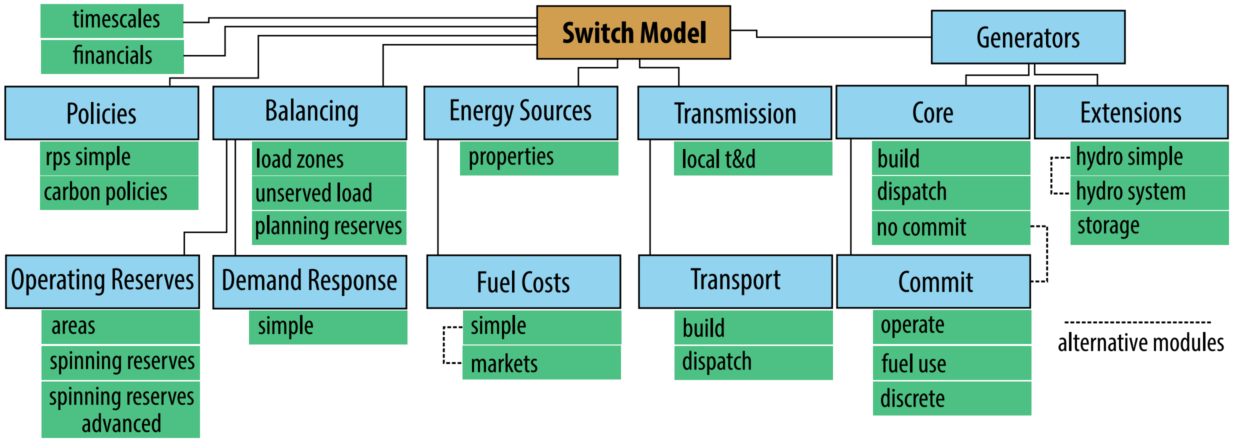


Figure 2: Package structure of the Switch model with list of modules.

- Uppercase calligraphic letters (e.g. $\mathcal{P}, \mathcal{T}, \mathcal{G}$) define sets (collections of similar items).
- Lowercase italic letters with subscripts (e.g. $c_p$) reference arbitrary model components, generally selected from dynamic sets of model components (details below).

Because Switch 2.0 contains many components, in this document we often use the same letter for multiple elements of a particular type, e.g., $B$ for decisions about the amount of capacity to build of any type of resource. When needed, we add a roman superscript to distinguish between these elements, e.g., $B^{\mathrm{G}}$ for the amount of generation capacity to build. Italic subscripts identify individual instances when there are multiple instances of a component indexed over a set, e.g., $B^{\mathrm{G}}_{g,p}$ for the amount of generation capacity to build in generation project $g$ during study period $p$ (in this case, $g$ is a member of the set of all generation projects $\mathcal{G}$ and $p$ comes from the set of study periods $\mathcal{P}$).

Note that components in the Switch 2.0 source code have longer names, more typical of a computer programming environment. These can generally be mapped directly to the math-style names used here, e.g., $B^{\mathrm{G}}_{g,p}$ translates to `BuildGen[g, p]` in the model code.

## 4.2 Overview

This section provides an overview of the mathematical formulation used by Switch 2.0. The precise formulation is determined by the set of modules included in a given run, as detailed in section 4.3.

### 4.2.1 Objective function

The objective function is defined by the `financials` module. It minimizes the net present value of all investment and operation costs:

$$\min \sum_{p \in \mathcal{P}} d_p \left\{ \sum_{c^{\mathrm{f}} \in \mathcal{C}^{\mathrm{fixed}}} c^{\mathrm{f}}_p + \sum_{t \in \mathcal{T}_p} w^{\mathrm{year}}_t \sum_{c^{\mathrm{v}} \in \mathcal{C}^{\mathrm{var}}} c^{\mathrm{v}}_t \right\} \tag{1}$$

Function (1) sums over sets of fixed costs $\mathcal{C}^{\mathrm{fixed}}$ and variable costs $\mathcal{C}^{\mathrm{var}}$. Each fixed cost component $c^{\mathrm{f}} \in \mathcal{C}^{\mathrm{fixed}}$ is a Pyomo object, indexed by investment period and specified in units of \$/year. This object may be a variable, parameter or expression (calculation based on other components). The term $c^{\mathrm{f}}_p$ is the element with index $p$ from component $c^{\mathrm{f}}$, i.e., a fixed cost that occurs during period $p$. Each variable cost component $c^{\mathrm{v}}$ is indexed by timepoint ($t$) and specified in units of \$/hour. Modules add components to the fixed and variable cost sets to represent each cost that they introduce. Hence, the exact equation will depend on which modules are selected by the user.

In most runs, fixed costs in $\mathcal{C}^{\mathrm{fixed}}$ include capital repayment for investments at a fixed financing rate over the lifetime of each asset, sunk costs from existing infrastructure, as well as fixed operating and maintenance (O&M) costs. Variable costs in $\mathcal{C}^{\mathrm{variable}}$ typically include fuel costs and variable O&M. The weight factor $w^{\mathrm{year}}_t$ scales costs from a sampled timepoint to an annualized value. The discount factor $d_p$ converts annualized costs from future periods to net present value.

### 4.2.2 Operational constraints

#### 4.2.2.1 Power balance

The `balancing.load_zones` module defines the main power balance requirement for the power system:

$$\sum_{p^{\mathrm{i}} \in \mathcal{P}^{\mathrm{inject}}} p^{\mathrm{i}}_{z,t} = \sum_{p^{\mathrm{w}} \in \mathcal{P}^{\mathrm{withdraw}}} p^{\mathrm{w}}_{z,t}, \qquad \forall z \in \mathcal{Z}, \forall t \in \mathcal{T} \tag{2}$$

Power injections and withdrawals in each load zone must be balanced during each timepoint. The power balance equation in (2) is expressed as an equality between two summations over dynamic sets of components that inject or withdraw power: $\mathcal{P}^{\mathrm{inject}}$ and $\mathcal{P}^{\mathrm{withdraw}}$. As with the objective function, modules add Pyomo objects to $\mathcal{P}^{\mathrm{inject}}$ and $\mathcal{P}^{\mathrm{withdraw}}$ to show the amount of power injected or withdrawn by each system component during each timepoint. Consequently the exact equation will depend on which modules are included. Objects in $\mathcal{P}^{\mathrm{inject}}$ and $\mathcal{P}^{\mathrm{withdraw}}$ are each indexed by load zone and timepoint and specified in units of MW.

Typically, the list of injections $\mathcal{P}^{\mathrm{inject}}$ includes power output $P_{g,t}$ for every generation project $g$ located in load zone $z$ and inward transmission flows into that load zone, $F_{\ell^{\mathrm{in}}_z,t}$. The list of withdrawals $\mathcal{P}^{\mathrm{withdraw}}$ typically includes customer loads $l_{z,t}$ and outward transmission flows $F_{\ell^{\mathrm{out}}_z,t}$.

The optional `balancing.operating_reserves.spinning_reserves` and `balancing.operating_reserves.spinning_reserves_advanced` modules define a similar balance for operating reserves.

#### 4.2.2.2 Dispatch

The `generators.core.dispatch` module defines fundamental components such as dispatched power $P_{g,t}$ and fuel consumption. It registers variable O&M with the objective function, but leaves it to other modules to model unit commitment and constrain fuel consumption to meaningful values.

The `generators.core.no_commit` module constrains dispatch based on installed capacity $K^{\mathrm{G}}_{g,p}$ (in MW) and an availability factor $\eta_{g,t}$:

$$0 \leq P_{g,t} \leq \eta_{g,t} K^{\mathrm{G}}_{g,p}, \qquad \forall \ell \in \mathcal{L}, p \in \mathcal{P}, \forall t \in \mathcal{T}_p \tag{3}$$

For firm generators, $\eta_{g,t}$ is time invariant and reflects average outage rates. For intermittent generators, $\eta_{g,t}$ also reflects the renewable availability timeseries. *No Commit* constrains fuel requirements based on dispatch and the generator's full load heat rate.

As an alternative to `generators.core.no_commit`, the `generators.core.commit` subpackage constrains dispatch $P_{g,t}$ based on committed capacity:

$$0 \leq W_{g,t} \leq \eta_g K^{\mathrm{G}}_{g,p}, \qquad \forall g \in \mathcal{G}, \forall p \in \mathcal{P}, \forall t \in \mathcal{T}_p \tag{4}$$

$$d^{\min}_g W_{g,t} \leq P_{g,t} \leq W_{g,t}, \qquad \forall g \in \mathcal{G}, \forall t \in \mathcal{T} \tag{5}$$

$$W_{g,t} - W_{g,t-1} = U_{g,t} - V_{g,t}, \qquad \forall g \in \mathcal{G}, \forall t \in \mathcal{T} \tag{6}$$

Eq. (4) limits committed capacity $W_{g,t}$ to available capacity (possibly multiple identical units) as defined by (3). Eq. (5) limits dispatch $P_{g,t}$ based on the generator's minimum dispatch fraction $d^{\min}_g$ and committed capacity. Eq. (6) defines startup and shutdown state-tracking variables ($U_{g,t}$ and $V_{g,t}$) as the change in committed capacity over time. The `generators.core.commit` module also registers one-time startup costs (fuel and O&M) per MW brought online. Ongoing fuel costs are determined by dispatch level and an optional piecewise linear incremental heat rate curve as described in Supplementary Material. An optional `generators.core.commit.discrete` module constrains committed capacity $W_{g,t}$ to discrete values based on the generator's unit size.

Transmission power flows receive similar treatment. The `transmission.transport` subpackage limits flows $F_{\ell,t}$ through a line $\ell$ based on available capacity $K^{\mathrm{L}}_{\ell,p}$ adjusted by the derating factor $\eta^{\mathrm{L}}_{\ell}$, as showed in Eq. (7).

$$0 \leq F_{\ell,t} \leq \eta^{\mathrm{L}}_{\ell} K^{\mathrm{L}}_{\ell,p}, \qquad \forall \ell \in \mathcal{L}, p \in \mathcal{P}, \forall t \in \mathcal{T}_p \tag{7}$$

#### 4.2.2.3 Minimum up and down times

The `generators.core.commit` module implements minimum up and down times rules by requiring that all capacity that was started up during a look-back window (equal to minimum uptime) is still on-line, and that capacity that was shutdown during the downtime look-back window remains uncommitted.

$$W_{g,t} \geq \sum_{t'=t-\hat{\tau}^{\mathrm{u}}_g}^{t} U_{g,t'}, \qquad \forall g \in \mathcal{G}, \forall t \in \mathcal{T} \tag{8}$$

$$W_{g,t} \leq \eta_g K^{\mathrm{G}}_{g,p(t)} - \sum_{t'=t-\hat{\tau}^{\mathrm{d}}_g}^{t} V_{g,t'}, \qquad \forall g \in \mathcal{G}, \forall t \in \mathcal{T} \tag{9}$$

where $\hat{\tau}_g$ is the number of prior timepoints to consider. To account for end-effects, Switch uses circular indexing for time series, so that $t = -1$ refers to the last timepoint in the same time series. This imposes a requirement that the system state at the end of each timeseries matches its starting state, which is equivalent to modeling each timeseries as an infinitely long sequence of identical series. This approach is best-suited for time series with a duration of a whole number of days.

#### 4.2.3 Investment constraints

##### 4.2.3.1 Power system construction

$$K^{\mathrm{G}}_{g,p} = \sum_{p' \in \mathcal{P}^{\mathrm{on}}_{g,p}} B^{\mathrm{G}}_{g,p'}, \qquad \forall g \in \mathcal{G}, \forall p \in \mathcal{P} \cup \{p_0\} \tag{10}$$

$$B^{\mathrm{G}}_{g,p} = b^{\mathrm{G}}_{g,p}, \qquad \forall g \in \mathcal{G}, \forall p \in \mathcal{P}^{\mathrm{G}}_g \tag{11}$$

$$K^{\mathrm{L}}_{\ell,p} = \sum_{p' \in \mathcal{P} \cup \{p_0\} : p' \leq p} B^{\mathrm{L}}_{p',k}, \qquad \forall \ell \in \mathcal{L}, \forall p \in \mathcal{P} \tag{12}$$

$$B^{\mathrm{L}}_{\ell,p} = b^{\mathrm{L}}_{\ell,p}, \qquad \forall \ell \in \mathcal{L}, \forall p \in \mathcal{P}^{\mathrm{L}}_\ell \tag{13}$$

Eqs. (10) and (12) define cumulative installed capacity for generation projects $K^{\mathrm{G}}_{g,p}$ and transmission lines $K^{\mathrm{L}}_{\ell,p}$ as of period $p$ as the sum of previous capacity additions $B^{\mathrm{G}}_{g,p'}$ and $B^{\mathrm{L}}_{\ell,p'}$, including existing infrastructure. For generation projects, the set $\mathcal{P}^{\mathrm{on}}_{g,p}$ lists all periods when capacity of type $g$ could have been built and still be in service in period $p$. Eqs. (11) and (13) fix the investment decisions of some generation projects and transmission lines over some periods $\mathcal{P}^{\mathrm{G}}_g$ and $\mathcal{P}^{\mathrm{L}}_\ell$ with predetermined values specified in input files (e.g. existing, planned, or preordained capacity).

##### 4.2.3.2 Maximum investment

$$0 \leq K^{\mathrm{G}}_{g,p} \leq \overline{k^{\mathrm{G}}}_g, \qquad \forall g \in \mathcal{G}^{\mathrm{rc}}, p \in \mathcal{P} \tag{14}$$

Eq. (14) constrains cumulative capacity for resource-constrained generators; generators where $\overline{k^{\mathrm{G}}}_g$ is defined.

The following sections provide complete details on all the standard modules included with Switch 2.0.

### 4.3 Switch modules

#### 4.3.1 timescales

In this module, different timescales are defined to be used in the model. Switch uses a three-level hierarchy of timescales to account for temporal dimension in various scales. These are:

- Periods: Set of multi-year timescales that describes when the investment decisions are taken. The duration of a period is typically on the order of one or more years, so costs associated with periods are specified in annualized costs. New assets are assumed to be added at the start of each period and available for use throughout the period.
- Timeseries: Set that denotes blocks of consecutive time points within a period. An individual time series could represent a single day, a week, a month or an entire year. Timeseries edge effects are addressed by treating the timeseries cyclically, so they typically have duration of a whole number of days within a single season so that ending conditions on 11:59pm of the last day in the series describes representative starting conditions for midnight on the first day in the series.
- Timepoints: Set that describes unique time steps within a time series. Timepoints are used to index exogenous variables such as electricity demand and renewable energy generation profiles. The duration of a time point is typically on the order of one or more hours, so costs associated with time points are specified in hourly units.

Table 1 summarizes the sets and parameters defined in this module:

| Type | Symbol | Description |
|---|---|---|
| Set | $\mathcal{P}$ | Set of all investment periods, indexed by $p$. |
| Parameter | $\text{st}_p$ | Year in which period $p$ begins. |
| Parameter | $y_p$ | Length in years of period $p$. |
| Set | $\mathcal{S}$ | Set of all time series. Indexed by $s$. |
| Subset | $\mathcal{S}_p$ | Subset of time series that fall in period $p$. |
| Parameter | $\text{num}_s$ | Number of time points in time series $s$. |
| Parameter | $\Delta_s$ | Duration in hours of each time point in time series $s$. Used for short-term thermodynamics such as energy storage calculations. |
| Parameter | $\theta_s$ | Number of times a time series $s$ (or equivalent conditions) occurs in its period. Used statistically for sample weighting for economics, pollution and long-term energy demand. |
| Set | $\mathcal{T}$ | Set of all time points, indexed by $t$. |
| Subset | $\mathcal{T}_s$ | Subset of time points that fall in time series $s$. |
| Subset | $\mathcal{T}_p$ | Subset of time points that fall in period $p$. |

Table 1: Model components defined in the `timescales` module.

With these parameters each timepoint's weight within the year is calculated as:

$$w_t^{\text{year}} = \Delta_s \cdot \theta_s / y_p, \qquad \forall t \in \mathcal{T}_s, \forall s \in \mathcal{S}_p, \forall p \in \mathcal{P}.$$

It is necessary to separate the components of the timepoint weight in order to accurately account for the short-term thermodynamics of energy storage within a representative day ($\Delta_s$) as well as statistical weighting ($\theta_s$) for total costs, pollution, aggregate energy demand, etc. Switch will check if the sum of total weights match the total hours in a period, that is in each period $p$:

$$\sum_{s \in \mathcal{S}_p} \text{num}_s \cdot \Delta_s \cdot \theta_s \approx \text{Total hours of } p, \qquad \forall p \in \mathcal{P}.$$

If this condition is not fulfilled, an error will be displayed, stopping the optimization. This check ensures an accurate weighting of variable vs. fixed costs.

### 4.3.2 financials

This module defines financial parameters and the objective function. These parameters are used to bring future costs to present or calculate annualized cost of investments. Table 2 summarizes the parameters defined in this module:

| Type | Symbol | Description |
|---|---|---|
| Parameter | $r$ | Annual real discount rate used to convert future dollars to present. |
| Parameter | $i$ | Annual real interest rate used to finance investments. |
| Parameter | baseyear | Base financial year in which future costs will be converted to net present value via discount rate $r$. |
| Set | $\mathcal{C}^{\text{fixed}}$ | Fixed cost components that contribute to the total cost in the cost-minimizing objective function. |
| Set | $\mathcal{C}^{\text{var}}$ | Variable cost components that contribute to the total cost in the cost-minimizing objective function. |

Table 2: Model components defined in the `financials` module.

This module also contains standard financial functions to convert from future to present value, determine the capital recovery factor to convert capital expenses into a series of uniform payments, etc. These are not shown here for brevity. This function also defines a cost-minimizing objective function. The modular structure of Switch makes it impossible to know all of the cost components at the time the code is written, because different modules will define different costs. To support a dynamic objective function that can be defined at runtime, two dynamic lists are created:

- Fixed costs components $\mathcal{C}^{\text{fixed}}$ is a set (defined as a Python list) of model components that contribute to overall system costs in each period. Each component $c^{\text{f}}$ in this set is a Pyomo object that is indexed by period $p$ and specified in units of annualized costs: non-discounted real dollars per year. Allowed Pyomo model components include parameters, decision variables, and expressions. Pyomo expressions are short calculations that are mathematically equivalent to fully constrained decision variables, except that expressions can be specified with fewer lines of code, appear to consume fewer computational resources and are completely factored out before sending the problem to the solver.

- Variable costs components $\mathcal{C}^{\text{var}}$ is a set (defined as a Python list) of model components that contribute to overall system costs on a timepoint basis. Each component $c^{\text{v}}$ in this list is a Pyomo object that is indexed by timepoint $t$ and specified in units of non-discounted real dollars per hour.

Thus, the objective function of the model can be written in an abstract form as:

$$\min \sum_{p \in \mathcal{P}} d_p \left\{ \sum_{c^{\text{f}} \in \mathcal{C}^{\text{fixed}}} c_p^{\text{f}} + \sum_{t \in \mathcal{T}_p} w_t^{\text{year}} \sum_{c^{\text{v}} \in \mathcal{C}^{\text{var}}} c_t^{v} \right\} \tag{15}$$

The objective function (15) minimizes the net present value of all investment and operation costs. The discount factor $d_p$ includes two components, one to convert annual payments during each period to an equivalent lump sum at the beginning of a period, and another to convert that lump sum to a net present value:

$$d_p = \frac{1 - (1 + r)^{-\text{y}_p}}{r} \cdot (1 + r)^{-(\text{st}_p - \text{baseyear})}$$

Each fixed cost component $c^{\text{f}}$ is a Pyomo object, indexed by period and specified in units of \$/year. This object may be a variable, parameter or expression (a calculation based on other components). The term $c_p^{\text{f}}$ is the element with index $p$ from component $c^{\text{f}}$. In the same way, variable cost components $c^{\text{v}}$ are indexed by timepoint and specified in units of \$/hour.

Depending on which modules are being used for a case study, different components will be added to each set. For example, the *storage* module defines new investment variables for the energy portion of storage rated in MWh of energy capacity with an associated unit cost. In the code, it defines an expression $\mathit{StorageEnergyInstallCosts}_p$ to summarize the annualized capital costs, and adds this expression to the list of fixed costs $\mathcal{C}^{\text{fixed}}$. In this formulation, storage has no variable cost, so the module does not add any components to $\mathcal{C}^{\text{var}}$. Switch's modular architecture allows users to select modules relevant to their study and keep other complexities out of the model and objective function. This can enable either faster execution, greater complexity, or greater time/spatial resolution elsewhere in the model. For example, in a single-bus study, investment and operational costs of transmission lines will not be included, and flow constraints will not even be defined. Removing those components can make the inclusion of discrete unit commitment or a larger time sample more practical.

#### 4.3.3 balancing.load_zones

In this module, the set of load zones are defined. Each load zone $z$ can represent either an electric bus, or a local area that can be approximated as a radial network attached to one central bus. Each load zone has associated a specific demand in each time point. Switch ensures that power is balanced in each load zone at each time point. Table 3 presents sets, parameters and variables defined in this module.

| Type | Symbol | Description |
|---|---|---|
| Set | $\mathcal{Z}$ | Set of all load zones, indexed by $z$. |
| Parameter | $l_{z,t}$ | Demand in MW at zone $z$ at time point $t$. |
| Subset | $\mathcal{Z}^{\text{peak}}$ | Subset of load zones that specify expected peak load at each period. |
| Parameter | $l_{z,p}^{\text{peak}}$ | Expected peak load demand in zone $z \in \mathcal{Z}^{\text{peak}}$ in period $p$ (optional). |
| Set | $\mathcal{P}^{\text{inject}}$ | Model components that inject power to the central bus of each load zone. |
| Set | $\mathcal{P}^{\text{withdraw}}$ | Model components that withdraw power from the central bus of each load zone. |

Table 3: Model components defined in the `balancing.load_zones` module.

In this module, the power balance equation is defined. Using the same approach as the objective function, two dynamic lists are created:

- Components that inject power $\mathcal{P}^{\text{inject}}$: It is a set (defined as a Python list) of components $p^{\text{i}}$ that contribute to a load zone balancing equation by injecting power. Each component in this list needs to be indexed by load zones $z$ and time points $t$, and must have units in MW.
- Components that withdraw power $\mathcal{P}^{\text{withdraw}}$: It is a set (defined as a Python list) of components $p^{\text{w}}$ that contribute to a load zone balancing equation by withdrawing power. Each component in this list needs to be indexed by load zones $z$ and time points $t$, and must have units in MW.

Thus, in a similar form as the objective function, the power balance equation can be written in abstract form as:

$$\sum_{p^{\mathrm{i}} \in \mathcal{P}^{\mathrm{inject}}} p^{\mathrm{i}}_{z,t} = \sum_{p^{\mathrm{w}} \in \mathcal{P}^{\mathrm{withdraw}}} p^{\mathrm{w}}_{z,t}, \qquad \forall z \in \mathcal{Z}, \forall t \in \mathcal{T} \tag{16}$$

As mentioned previously for the case of the objective function, depending on which modules are being used for a specific case study, different components will be added to each list. For example, in this module, demand $l_{z,t}$ will be added as a component that withdraws power $\mathcal{P}^{\mathrm{withdraw}}$ for each zone at each time point.

#### 4.3.4 energy_sources.properties

In this module, all energy sources are defined for the Switch model. All generation projects are required to define their energy source. This is useful to obtain the final energy mix and ensure the requirements of renewable portfolio standards. Table 4 presents sets and parameters defined in this module.

| Type | Symbol | Description |
|---|---|---|
| Set | $\mathcal{E}$ | Set of all energy sources, indexed by $f$. |
| Subset | $\mathcal{E}^{\mathrm{F}}$ | Subset of all fuel-baseed energy sources. |
| Subset | $\mathcal{E}^{\mathrm{R}}$ | Subset of all non-fuel energy sources. |
| Parameter | $\xi_f, f \in \mathcal{E}^{\mathrm{F}}$ | Direct emissions of CO2 of a fuel in tCO2/MMBtu. |
| Parameter | $\mu_f, f \in \mathcal{E}$ | Emissions attributable to an energy-source before it is consumed in tCO2/MMBtu. |

Table 4: Model components defined in the `energy_sources.properties` module.

#### 4.3.5 generators.core.build

In this module all generation projects that have been built, could be expanded or could potentially be built are defined. Table 5 presents sets, parameters and variables that are defined in this module.

| Type | Symbol | Description |
|---|---|---|
| Set | $\mathcal{G}$ | Set of all generation projects, indexed by $g$. |
| Subset | $\mathcal{G}^{\mathrm{B}}$ | Subset of all generation projects that are baseload. |
| Subset | $\mathcal{G}^{\mathrm{F}}$ | Subset of all generation projects that are fueled powered. |
| Subset | $\mathcal{G}^{\mathrm{R}}$ | Subset of all generation projects that are variable renewable. |
| Subset | $\mathcal{G}^{\mathrm{rc}}$ | Subset of all generation projects that are resource constrained. |
| Subset | $\mathcal{G}^{\mathrm{Z}}_z$ | Subset of all generation projects that are located in load zone $z$. |
| Parameter | $b^{\mathrm{unit}}_g$ | Size of individual generating units within project $g$ (optional). |
| Subset | $\mathcal{G}^{\mathrm{unit}}$ | Subset of generation projects for which a discrete unit size $\mathrm{b}^{\mathrm{unit}}_g$ has been specified. |
| Subset | $\mathcal{E}^{\mathrm{F}}_g$ | Subset of fuels that can be used by generator $g$. |
| Parameter | $\mathrm{by}_g$ | Earliest year in which construction or expansion of capacity in project $g$ can occur. |
| Parameter | $\mathrm{ly}^{\mathrm{G}}_g$ | Lifetime over which capital investment in generation project $g$ will be recovered (years). |
| Parameter | $b^{\mathrm{G}}_{g,p}$ | Predetermined installed capacity of project $g$ at period $p$ (MW). |
| Subset | $\mathcal{P}^{\mathrm{GB}}_g$ | Subset of periods during which capacity may be added in generation project $g$. |
| Subset | $\mathcal{P}^{\mathrm{GD}}_g$ | Subset of periods for which the capacity additions in project $g$ are predetermined (may include years before the main study). |
| Subset | $\mathcal{P}^{\mathrm{on}}_{g,p}$ | Subset of previous periods of $p$ (including period $p$) in which the installed capacity of the generation project $g$ is online. This subset does not include capacity that is already retired. |
| Parameter | $\overline{k^{\mathrm{G}}}_g$ | Maximum allowed capacity for project $g$. |
| Subset | $\mathcal{P}^{\mathrm{on}}_g$ | Subset of periods when generation project $g$ may have capacity online. This excludes periods before $g$ can be built or after it must be retired. |
| Subset | $\mathcal{T}^{\mathrm{on}}_g$ | Subset of timepoints when generation project $g$ may have capacity online. Corresponds to $\mathcal{P}^{\mathrm{on}}_g$. |
| Parameter | $\overline{k^{\mathrm{G}}}_g$ | Maximum allowed capacity for project $g$. |
| Variable | $B^{\mathrm{G}}_{g,p}$ | Amount of capacity built (added) in project $g$ in period $p \in \mathcal{P}^{\mathrm{GB}}_g$. |
| Variable | $K^{\mathrm{G}}_{g,p}$ | Cumulative capacity of project $g$ as of period $p$. |
| Parameter | $\hat{c}^{\mathrm{G,inv}}_g$ | Overnight capital cost per MW to install this project on the build year $\mathrm{by}_g$. |
| Parameter | $c^{\mathrm{G,fix}}_g$ | Fixed Operation and Maintenance annualized costs per MW of built capacity. |
| Parameter | $\hat{c}^{\mathrm{G,upg}}_g$ | Overnight cost of grid upgrades to support the project $g$ per MW installed. |

Table 5: Model components defined in the `generators.core.build` module.

Note that in general in Switch, a generation project $g$ represents a "stack" of multiple identical generating units in the same load zone, where the $B$ and $K$ variables can exceed the size of one unit (commitment and dispatch logic use this approach as well). This aggregation sharply reduces memory requirements in large models. It is also possible to model units individually by setting $\overline{k^{\mathrm{G}}}_g$ and/or $b^{\mathrm{G}}_{g,p}$ to the size of one generating unit.

Constraints regarding the investment decisions are also defined in this module:

$$K^{\mathrm{G}}_{g,p} = \sum_{p' \in \mathcal{P}^{\mathrm{on}}_{g,p}} B^{\mathrm{G}}_{g,p'}, \qquad \forall g \in \mathcal{G}, \forall p \in \mathcal{P} \cup \{p_0\} \tag{17}$$

$$B^{\mathrm{G}}_{g,p} = b^{\mathrm{G}}_{g,p}, \qquad \forall g \in \mathcal{G}, \forall p \in \mathcal{P}^{\mathrm{GD}}_g \tag{18}$$

$$K^{\mathrm{G}}_{g,p} \leq \overline{k^{\mathrm{G}}}_g, \qquad \forall g \in \mathcal{G}^{\mathrm{rc}}, \forall p \in \mathcal{P} \tag{19}$$

$$0 \leq B^{\mathrm{G}}_{g,p}, \qquad \forall g \in \mathcal{G}, \forall p \in \mathcal{P}^{\mathrm{GB}}_g \tag{20}$$

Equation (17) shows that cumulative installed capacity is defined by the sum of previous and current-period installed capacity. With this, expansions that are decided on one period will be available in the same period. Capacity that is retired before period $p'$ will not be considered in equation (17). Equation (18) fixes the decision of built capacity for some periods that are predetermined, either for legacy projects ($p'$ in the past) or for future projects. Equation (19)

limits the maximum installed capacity for generation projects that are resource limited, such as wind farms or geothermal fields. Finally equation (20) forces nonnegativity of the build decisions.

Overnight capital costs $\hat{c}$ are annualized using the interest rate $i$:

$$c_g^{\mathrm{G,inv}} = \left( \frac{i}{1-(1-i)^{-\mathrm{ly}_g^{\mathrm{G}}}} \right) \hat{c}_g^{\mathrm{G,inv}}$$

$$c_g^{\mathrm{G,upg}} = \left( \frac{i}{1-(1-i)^{-\mathrm{ly}_g^{\mathrm{G}}}} \right) \hat{c}_g^{\mathrm{G,upg}}$$

Then, the terms $(c_g^{\mathrm{G,inv}} + c_g^{\mathrm{G,upg}})B_{g,p}^{\mathrm{G}}$ and $c_g^{\mathrm{G,fix}} B_{g,p}^{\mathrm{G}}$ are added to the set $\mathcal{C}^{\mathrm{fixed}}$ for each project and period in order to be considered in the objective function (15).

#### 4.3.6 generators.core.gen_discrete_build

This optional module allows users to prevent construction of partial units of generation technologies that have a discrete unit size $b_g^{\mathrm{unit}}$ specified. For this purpose a non-negative integer variable $B_{g,p}^{\mathrm{int}} \in \mathbb{Z}_0^+$ is defined for the set of generators for which a unit size has been specified $\mathcal{G}^{\mathrm{unit}}$.

Then, forcing the build variable to be a multiple of its unit size, a discrete formulation is implemented:

$$B_{g,p}^{\mathrm{G}} = b_g^{\mathrm{unit}} B_{g,p}^{\mathrm{int}}, \qquad \forall g \in \mathcal{G}^{\mathrm{unit}}, \forall p \in \mathcal{P} \tag{21}$$

#### 4.3.7 generators.core.dispatch

Table 6 presents parameters and variables defined in this module:

| Type | Symbol | Description |
|---|---|---|
| Variable | $P_{g,t}$ | Average power in MW produced by project $g$ during timepoint $t$. |
| Variable | $R_{g,t,f}$ | Rate of use of fuel $f \in \mathcal{E}_g^{\mathrm{F}}$ by project $g \in \mathcal{G}^{\mathrm{F}}$ during timepoint $t$ (in MMBtu/h). Each generator may use multiple fuels. |
| Parameter | $\eta_g$ | Fraction of a time a project $g \in \mathcal{G}$ is expected to be available (used to de-rate for forced outages). |
| Parameter | $\eta_{g,t}$ | Maximum possible output from renewable project $g \in \mathcal{G}^{\mathrm{R}}$ in timepoint $t$ (per-unit). |
| Parameter | $h_g$ | Full load heat rate (inverse of thermal efficiency), in MMBtu per MWh. |
| Parameter | $c_g^{\mathrm{om}}$ | Variable operations and maintenance costs per MWh of power produced by project $g$. |

Table 6: Model components defined in the `generators.core.dispatch` module.

The sum of all projects' dispatch at each timepoint $t$ in each load zone $z$ is added to the dynamic list $\mathcal{P}^{\mathrm{inject}}$ in order to be included in the power balance equation (16). Variable O&M costs $c_g^{\mathrm{om}} P_{g,t}$ are added to the list $\mathcal{C}^{\mathrm{var}}$ to be included in the objective function (15).

The cost of operating fuel-powered generators also depends on the generators' heat rates (which may vary depending on operating level) and fuel prices (which may vary by period or have their own market structure). The fuel use rates $R_{g,t,f}$ are constrained to match the power output $P_{g,t}$ for each generator during each timepoint by the `generators.core.no_commit` or `generators.core.commit.fuel_use` module. The `energy_sources.fuel_costs.simple` or `energy_sources.fuel_costs.markets` module calculates costs associated with the fuel use $R_{g,t,f}$.

#### 4.3.8 energy_sources.fuel_costs.simple

This module defines a simple formulation with flat fuel costs. This module is mutually exclusive with the `energy_sources.fuel_costs.fuel_markets` module. Table 7 presents the sets and parameters defined in this module.

| Type | Symbol | Description |
|---|---|---|
| Parameter | $c^{\text{fuel}}_{z,f,p}$ | Cost per MMBtu for fuel $f$ in load zone $z$ during period $p$. |
| Set | $\mathcal{F}^{\text{unav}}$ | Set of tuples of (project $g$, timepoint $t$, fuel $f$) where fuel $f$ is not available. |

Table 7: Model components defined in the `energy_sources.fuel_costs.simple` module.

Total fuel costs for each zone and timepoint are calculated using the expression

$$\sum_{g\in\mathcal{G}^{\text{Z}}_z:t\in\mathcal{T}^{\text{on}}_g}\ \sum_{f\in\mathcal{E}^{\text{F}}_g} c^{\text{fuel}}_{z,f,p(t)} \times R_{g,t,f}, \qquad \forall z\in\mathcal{Z}, t\in\mathcal{T}. \tag{22}$$

These are added to the dynamic list $\mathcal{C}^{\text{var}}$ for inclusion in the objective function (15).

Fuel use rate is constrained to zero if no fuel is available for a generation project:

$$R_{g,t,f} = 0, \qquad \forall (g,t,f)\in\mathcal{F}^{\text{unav}} \tag{23}$$

#### 4.3.9 energy_sources.fuel_costs.markets

This module defines model components to describe fuel markets. Table 8 presents sets, parameters and variables defined in this module:

| Type | Symbol | Description |
|---|---|---|
| Set | $\mathcal{M}$ | Set of all regional fuel markets (rfm), indexed by $m$. |
| Parameter | $f^{\text{M}}_m$ | Fuel that is sold in the regional fuel market $m$. |
| Subset | $\mathcal{Z}^{\text{M}}_m$ | Set of all load zones served by the regional fuel market $m$. |
| Set | $\Sigma_{m,p}$ | Set of supply tiers (i.e., complete supply curve) for a given regional fuel market $m$ and period $p$, indexed by $\sigma$. |
| Set | $\mathcal{F}^{\text{unav}}$ | Set of tuples of (project $g$, timepoint $t$, fuel $f$) where fuel $f$ is not available. |
| Parameter | $c^{\text{fuel}}_\sigma$ | Cost of a fuel in a particular tier of a supply curve $\sigma$. |
| Parameter | $\text{limit}_\sigma$ | Annual limit of a fuel available for a particular tier in the supply curve $\sigma$. |
| Variable | $R^{\text{tier}}_\sigma$ | The annual rate of fuel consumption in each tier of a supply curve, $\sigma\in\Sigma_{m,p}$, in MMBtu/year. |

Table 8: Model components defined in the `energy_sources.fuel_costs.markets` module.

Each regional fuel market has a supply curve with discrete tiers of escalating costs. Tiered supply curves are a flexible format that allows anything from a flat cost in every load zone with no limits on consumption, to a detailed supply curve of fuel for each load zone. For example, to specify a simple biomass flat cost, a user would place all load zones into a single regional fuel market and specify a single-tier supply curve with no upper limit. To specify a detailed biomass supply curve, the user would assign each load zone to a distinct biomass regional fuel market and specify multiple tiers in each market, where each tier has an upper bound. (A `fuel_market_expansion` module in

the Hawaii regional subpackage also allows capital investments to expand the capacity available in each tier, e.g., via construction of new fuel-delivery infrastructure.)

Constraints regarding the tier limits and linkage with power production are defined in this module:

$$0 \leq R_{\sigma}^{\text{tier}} \leq \text{limit}_{\sigma}, \qquad \forall p \in \mathcal{P}, \forall m \in \mathcal{M}, \forall \sigma \in \Sigma_{m,p} \tag{24}$$

$$\sum_{\sigma \in \Sigma_{m,p}} R_{\sigma}^{\text{tier}} = \sum_{z \in \mathcal{Z}_m^{\text{M}}} \sum_{g \in \mathcal{G}_z^{\text{Z}} : f_m^{\text{M}} \in \mathcal{E}_g^{\text{F}}} \sum_{t \in \mathcal{T}_p \cap \mathcal{T}_g^{\text{on}}} w_t^{\text{year}} R_{g,t,f}, \qquad \forall m \in \mathcal{M}, \forall p \in \mathcal{P} \tag{25}$$

$$R_{g,t,f} = 0, \qquad \forall (g,t,f) \in \mathcal{F}^{\text{unav}} \tag{26}$$

Equation (24) limits the fuel consumption in each tier of each fuel market supply curve. Equation (25) connects total activity in the supply market with consumption of the corresponding fuel by generators in the corresponding load zones. Finally (26) forces the consumption rate to zero if a fuel is unavailable for a generation project.

Total fuel costs of all tiers of a supply curve from all regional fuel markets during period $p$ are calculated as follows:

$$\text{AnnualFuelCosts}_p = \sum_{m \in \mathcal{M}} \sum_{\sigma \in \Sigma_{m,p}} c_{\sigma}^{\text{fuel}} \cdot R_{\sigma}^{\text{tier}}, \qquad \forall p \in \mathcal{P}$$

These are added to the set $\mathcal{C}^{\text{fixed}}$ in order to be considered in the objective function (15).

#### 4.3.10 transmission.transport.build

This module and `transmission.transport.dispatch` define bulk transmission capability for an electric power system using a "transport model." This consists of corridors or flowgates connecting load zones, with finite transfer capability through each corridor. Switch is allowed to expand available transfer capability (capacity) along each corridor, subject to limits set by the user. This approach is intended to represent the capabilities of the network and the cost of expanding those capabilities, without constructing a detailed electrical model of the network. These modules are optional; for copperplate models, users may place all generation and load in a single load zone and omit the transmission modules.

Table 9 presents sets, parameters and variables defined in `transmission.transport.build`:

| Type | Symbol | Description |
|---|---|---|
| Set | $\mathcal{L}$ | Set of all transmission corridors, indexed by $\ell$. |
| Parameter | $\zeta_\ell^1$ | Load zone at the start of corridor $\ell$. |
| Parameter | $\zeta_\ell^2$ | Load zone at the end of corridor $\ell$. |
| Parameter | $\mathrm{km}_\ell$ | Length in km of transmission corridor $\ell$. |
| Parameter | $\eta_\ell^L$ | Overall derating factor for transmission corridor $\ell$ that can reflect forced outage rates, stability or contingency limitations. |
| Parameter | $\eta_\ell^{\mathrm{L,ef}}$ | Efficiency; proportion of power sent through corridor $\ell$ that reaches the other end. |
| Subset | $\mathcal{P}_\ell^{\mathrm{L}}$ | Subset of periods in which capacity expansion in transmission corridor $\ell$ is predetermined (may include years before start of the study) |
| Parameter | $b_{\ell,p}^{\mathrm{L}}$ | Predetermined expansion of transfer capability in corridor $\ell$ during period $p \in \mathcal{P}_\ell^{\mathrm{L}}$. |
| Variable | $B_{\ell,p}^{\mathrm{L}}$ | Transfer capability added in corridor $\ell$ during period $p$ (MW). |
| Variable | $K_{\ell,p}^{\mathrm{L}}$ | Cumulative transfer capability through transmission corridor $\ell$ as of period $p$. |
| Parameter | $\overline{b^{\mathrm{L}}}_\ell$ | Maximum expansion of transfer capacity per period for corridor $\ell$ (MW). |
| Parameter | $\hat{c}^{\mathrm{L}}$ | Generic cost of expanding transfer capability in units of \$(BaseYear) per MW per km. |
| Parameter | $\alpha_\ell$ | Cost multiplier for expanding capacity on a specific corridor $\ell$. |
| Parameter | $\beta$ | Describes the fixed O&M costs per year as a fraction of capital costs. |
| Parameter | $\mathrm{ly}_\ell^{\mathrm{L}}$ | Lifetime over which capital costs are recovered for line $\ell$ (years). |

Table 9: Model components defined in the `transmission.transport.build` module.

With these parameters it is possible to calculate the annualized carrying cost (capital and O&M) per MW of capacity in transmission corridor $\ell$:

$$c_\ell^{\mathrm{L,inv}} = \left(\frac{i}{1-(1-i)^{-\mathrm{ly}_\ell^{\mathrm{L}}}}\right)\hat{c}^{\mathrm{L}} \cdot \alpha_\ell \cdot \mathrm{km}_\ell$$
$$c_\ell^{\mathrm{L,fix}} = \beta c_\ell^{\mathrm{L,inv}}$$

These costs are multiplied by the installed transmission capacity as of each future period, $K_{\ell,p}^{\mathrm{L}}$, then discounted to the base year, and added to the set $\mathcal{C}^{\mathrm{fixed}}$ for inclusion in the objective function (15).

New constraints are added in this module, such as the maximum allowed transmission expansion per period.

$$K_{\ell,p}^{\mathrm{L}} = \sum_{p' \le p} B_{\ell,k}^{\mathrm{L}}, \qquad \forall \ell \in \mathcal{L}, \forall p \in \mathcal{P} \cup \{p_0\} \tag{27}$$
$$B_{\ell,p}^{\mathrm{L}} = b_{\ell,p}^{\mathrm{L}}, \qquad \forall \ell \in \mathcal{L}, \forall p \in \mathcal{P}_\ell^{\mathrm{L}} \tag{28}$$
$$0 \le B_{\ell,p}^{\mathrm{L}} \le \overline{b^L}_\ell, \qquad \forall \ell \in \mathcal{L}, \forall p \in \mathcal{P} \tag{29}$$

#### 4.3.11 transmission.transport.dispatch

This module models the operation of a transmission system represented as a transport model (also see `transmission.transport.build`. Table 10 presents sets, parameters and variables in this module:

| Type | Symbol | Description |
|---|---|---|
| Set | $\mathcal{L}^{\mathrm{D}}$ | Set of directed transmission corridors. It is constructed with the ordered combinations of $\zeta_\ell^1$ with $\zeta_\ell^2$ based on $\mathcal{L}$, and is indexed by $\ell^{\mathrm{d}}$ |
| Set | $\mathcal{L}_z^{\mathrm{in}}$ | Set of directed transmission corridors where flows are directed into zone $z$, indexed by $\ell_z^{\mathrm{in}}$. |
| Set | $\mathcal{L}_z^{\mathrm{out}}$ | Set of directed transmission corridors where flows are directed out of zone $z$, indexed by $\ell_z^{\mathrm{out}}$. |
| Variable | $F_{\ell^{\mathrm{d}},t}$ | Power flow through a directed corridor $\ell^{\mathrm{d}}$. $F_{\ell_z^{\mathrm{in}},t}$ and $F_{\ell_z^{\mathrm{out}},t}$ reflect power flowing into or out of a particular load zone. |

Table 10: Model components defined in the `transmission.transport.dispatch` module.

The constraint of maximum flow through lines is defined as:

$$0 \leq F_{\ell^{\mathrm{d}},t} \leq \eta^{\mathrm{L}}_{\ell(\ell^{\mathrm{d}})} K_{\ell(\ell^{\mathrm{d}}),p}, \qquad \forall \ell^{\mathrm{d}} \in \mathcal{L}^{\mathrm{D}}, \forall p \in \mathcal{P}, \forall t \in \mathcal{T}_p \tag{30}$$

Note that this formulation generates two flow variables per corridor, one to define the flow going from $\zeta_\ell^1$ to $\zeta_\ell^2$, and the other to define the flow going from $\zeta_\ell^2$ to $\zeta_\ell^1$. The efficiency of a corridor only affects the flows being received from a line $\ell$ in a zone $z$, and not the sending flows.

With this approach, total inflows to zone $z$ from all other zones can be calculated as:

$$F_z^{\mathrm{in}} = \sum_{\ell \in \mathcal{L}_z^{\mathrm{in}}} \eta_\ell^{\mathrm{L,ef}} F_{\ell,t} \qquad \forall z \in \mathcal{Z} \tag{31}$$

$F_z^{\mathrm{in}}$ is added to the set of power-injecting components $\mathcal{P}^{\mathrm{inject}}$ for inclusion in the power balance equation (16).

Total outflow from zone $z$ can be calculated as:

$$F_z^{\mathrm{out}} = \sum_{\ell \in \mathcal{L}_z^{\mathrm{out}}} F_{\ell,t} \qquad \forall z \in \mathcal{Z} \tag{32}$$

$F_z^{\mathrm{out}}$ is added to the set of power-withdrawing components $\mathcal{P}^{\mathrm{withdraw}}$ for inclusion in the power balance equation (16).

#### 4.3.12 generators.core.no_commit

This module defines simple limitations on project dispatch without explicitly committing generating units. This module is mutually exclusive with `unit commit` module which constrains dispatch using unit commitment decisions.

Table 11 presents the variable defined in this module:

| Type | Symbol | Description |
|---|---|---|
| Variable | $P^{\mathrm{B}}_{p,t}$ | Amount of power to produce from baseload generator $g \in \mathcal{G}^{\mathrm{B}}$ at all times during period $p \in \mathcal{P}_g^{\mathrm{on}}$ (MW) |

Table 11: Model components defined in the `generators.core.no_commit`.

In this module, constraints regarding upper and lower dispatch limits are defined, depending on the type of project:

$$P_{g,t} = P^{\mathrm{B}}_{g,p(t)}, \qquad \forall g \in \mathcal{G}^{\mathrm{B}}, \forall t \in \mathcal{T}_g^{\mathrm{on}} \tag{33}$$

$$0 \le P_{g,t} \le \eta_g K^{\mathrm{G}}_{g,p(t)}, \qquad \forall g \in \mathcal{G} - \mathcal{G}^{\mathrm{R}}, \forall t \in \mathcal{T}^{\mathrm{on}}_g \tag{34}$$

$$0 \le P_{g,t} \le \eta_g \eta_{g,t} K^{\mathrm{G}}_{g,p(t)}, \qquad \forall g \in \mathcal{G}^{\mathrm{R}}, \forall t \in \mathcal{T}^{\mathrm{on}}_g \tag{35}$$

$$\sum_{f \in \mathcal{E}^{\mathrm{F}}_g} R_{g,t,f} = h_g P_{g,t}, \qquad \forall g \in \mathcal{G}^{\mathrm{F}}, \forall t \in \mathcal{T}^{\mathrm{on}}_g \tag{36}$$

See `generators.core.build` for definitions of the indexing sets used here and `generators.core.dispatch` for the variables and parameters. Constraint (33) forces the dispatch of baseload projects at a fixed level throughout each period (i.e., the model can decide whether to have them online or not each period, but not ramp them up and down). Equation (34) defines the upper limit for standard generation projects. Equation (35) limits the maximum dispatch of renewable projects depending on their capacity and availability at each time point. Finally, equation (36) calculates fuel consumption for fuel-powered generators using the full load heat rate.

#### 4.3.13 generators.core.commit.operate

This module defines model components for a linear unit commitment (UC) of generation projects. In this context, "linear" means that fractional parts of a generation project can be committed. This provides fast analysis which is reasonably accurate for large power systems, where the inaccuracy is small relative to the size of the generation fleet. If discrete unit commitment is needed (committing projects in full-unit chunks), users can include the optional `generators.core.commit.discrete` module, discussed below.

This module must be used with `generators.core.commit.fuel_use`, which defines corresponding fuel-use terms. This module is mutually exclusive with the `generators.core.no_commit` module, which constrains dispatch to simple upper and lower limits.

Note that all of Switch's unit-commitment and reserve calculations are designed to work with generation projects $g$ that represent either a single generating unit or a stack of multiple identical units. Using stacked projects significantly reduces memory requirements and model complexity without compromising fidelity. This approach assumes that all committed units in the same project are dispatched at the same level, which is a least-cost operating strategy.

Table 12 presents the variables and parameters defined in the `generators.core.commit.operate` module:

| Type | Symbol | Description |
|---|---|---|
| Variable | $W_{g,t}$ | How much capacity to commit (have online) in project $g$ in timepoint $t \in \mathcal{T}^{\mathrm{on}}_g$. |
| Variable | $U_{g,t}$ | How much additional capacity to commit (startup) in project $g$ in timepoint $t \in \mathcal{T}^{\mathrm{on}}_g$. |
| Variable | $V_{g,t}$ | How much committed capacity to decommit (shutdown) in project $g$ in timepoint $t \in \mathcal{T}^{\mathrm{on}}_g$. |
| Parameter | $d^{\mathrm{min}}_g$ | Minimum dispatch fraction (minimum load) of the committed capacity (defaults to 1 for baseload projects, 0 for others). |
| Parameter | $c^{\mathrm{up,OM}}_g$ | Variable O&M costs per MW for starting up capacity. |
| Parameter | $c^{\mathrm{up,fuel}}_g$ | Fuel costs per MW for starting up capacity. |
| Parameter | $\delta^{\mathrm{up,fuel}}_g$ | Fuel requirements for starting up additional generation capacity, in units of MMBtu/MW. |
| Parameter | $\tau^{\mathrm{u}}_g$ | Minimum time that generator $g$ can be committed (up, online) in hours. |
| Parameter | $\tau^{\mathrm{d}}_g$ | Minimum time that generator $g$ can be uncommitted (down, offline) in hours. |

Table 12: Model components defined in the `generators.core.commit.operate` module.

In the UC setting, several constraints must be defined: maximum commitment for each project is limited by the available capacity, while the dispatch is limited by the amount of capacity committed.

$$0 \le W_{g,t} \le \eta_g K^{\mathrm{G}}_{g,p(t)}, \qquad \forall g \in \mathcal{G}, \forall t \in \mathcal{T}^{\mathrm{on}}_g \tag{37}$$
$$d^{\min}_g W_{g,t} \le P_{g,t}, \qquad \forall g \in \mathcal{G}, \forall t \in \mathcal{T}^{\mathrm{on}}_g \tag{38}$$
$$P_{g,t} \le W_{g,t}, \qquad \forall g \in \mathcal{G} - \mathcal{G}^{\mathrm{R}}, \forall t \in \mathcal{T}^{\mathrm{on}}_g \tag{39}$$
$$P_{g,t} \le \eta_{g,t} W_{g,t}, \qquad \forall g \in \mathcal{G}^{\mathrm{R}}, \forall t \in \mathcal{T}^{\mathrm{on}}_g \tag{40}$$
$$W_{g,t} - W_{g,t-1} = U_{g,t} - V_{g,t}, \qquad \forall g \in \mathcal{G}, \forall t \in \mathcal{T}^{\mathrm{on}}_g \tag{41}$$

Equation (37) limits the maximum commitment to be lower than the available capacity. Equations (38)-(40) force the dispatch to fall between the minimum and maximum load for the committed capacity. Finally constraint (41) provides consistency between the commitment level and the startup and shutdown variables.

Minimum up and minimum down times rules are enforced by requiring that all capacity that was started up during a lookback window (equal to minimum uptime) is still online, and all capacity that was shutdown during the downtime lookback window is still offline:

$$W_{g,t} \ge \sum_{t'=t-\hat{\tau}^{\mathrm{u}}_g}^{t} U_{g,t'}, \qquad \forall g \in \mathcal{G}, \forall t \in \mathcal{T} \tag{42}$$

$$\eta_g K^{\mathrm{G}}_{g,p(t)} - W_{g,t} \ge \sum_{t'=t-\hat{\tau}^{\mathrm{d}}_g}^{t} V_{g,t'}, \qquad \forall g \in \mathcal{G}, \forall t \in \mathcal{T} \tag{43}$$

in which $\hat{\tau}_g = \mathrm{round}\{\tau_g/\Delta_{s(t)}\}$ (i.e., the lookback window is rounded to the nearest whole number of timesteps).

The startup operation and maintenance costs for each generator at each timepoint are converted to an hourly rate as $c^{\mathrm{up,OM}}_g \cdot U_{g,t}/\Delta_{s(t)}$ and then added to the set $\mathcal{C}^{\mathrm{var}}$ for inclusion in the objective function (15). Startup fuel is addressed by `generators.core.commit.fuel_use`.

#### 4.3.14 generators.core.commit.discrete

This optional module allows users to require discrete unit commitment, where projects are committed in chunks equal to the size of individual generating units. This is done by defining an integer variable $W^{\mathrm{int}}_{g,t} \in \mathbb{Z}^+_0$ and a discrete size for each generating unit $b^{\mathrm{unit}}_g$ in MW. All projects with $b^{\mathrm{unit}}_g$ defined are added to the set $\mathcal{G}^{\mathrm{unit}}$. Then a discrete formulation is implemented by forcing the commitment variable to be a multiple of the unit size:

$$W_{g,t} = \eta_g \cdot b^{\mathrm{unit}}_g \cdot W^{\mathrm{int}}_{g,t}, \qquad \forall g \in \mathcal{G}^{\mathrm{unit}}, \forall t \in \mathcal{T}^{\mathrm{on}}_g \tag{44}$$

#### 4.3.15 generators.core.commit.fuel_use

This module describes fuel use, including the interactions between unit commitment, dispatch and part-load heat rates (efficiency). This module must be used with `generators.core.commit.operate`.

In general, fuel requirements for most generators can be approximated very well using a simple proportionality between fuel usage and power production, i.e., the full-load heat rate. However, when more operational detail is needed the standard is to model fuel consumption via a convex, piecewise-linear heat rate curve. This consists of several line segments that have increasing slopes. Accurate estimates of fuel usage are particularly important in systems with high fuel prices or strict carbon caps or carbon taxes.

Each line segment of fuel usage has an increasing slope in units of MMBtu/h/MW when more power is being generated. If fuel has a cost associated with it, in a cost minimizing problem, if the fuel usage variable is greater than or equal to each segment line, it will be reduced till it touches one of the segments. Note that this method requires that heat rates increase with the energy production so the lines collectively form a convex boundary for fuel usage.

Table 13 presents the sets, parameters and variables defined in this module:

| Type | Symbol | Description |
|---|---|---|
| Set | $\mathcal{U}_g$ | Set of ordered segments lines used for defining the heat rate curve of project $g$, indexed by $u$. |
| Parameter | $p_{g,u}^{\min}$ | Minimum power in MW of segment line $u$ of project $g$. |
| Parameter | $p_{g,u}^{\max}$ | Maximum power in MW of segment line $u$ of project $g$. It is required that $P_u^{\max} = P_{u+1}^{\min}$. |
| Parameter | $\gamma_g$ | Fuel use rate in MMBtu/h at minimum power of project $g$. |
| Parameter | $\delta_{g,u}$ | Incremental heat rate in MMBtu/MWh for segment line $u$ of project $g$. |
| Parameter | $n_{g,u}$ | Normalized $y$-intercept in MMBtu/(h · MW-capacity) of the segment $u$ of project $g$. Derived from $p_{g,u}^{\min}, p_{g,u}^{\max}, \gamma_g$ and $\delta_{g,u}$. |

Table 13: Model components defined in the `generators.core.commit.fuel_use` module.

For each segment line $u$, a constraint of fuel use in MMBtu/h for each project $g$ at time point $t$ is defined as:

$$R_{g,t,f} \geq \frac{1}{\Delta_{s(t)}}(\delta_g^{\text{up,fuel}} \cdot U_{g,t}) + n_{g,u} \cdot W_{g,t} + \delta_{g,u} \cdot P_{g,t}, \quad \forall g \in \mathcal{G}^{\text{F}}, \forall t \in \mathcal{T}, \forall f \in \mathcal{E}_g^{\text{F}}, \forall u \in \mathcal{U}_g \quad (45)$$

As an example, input data for generator $g$ must be formatted as:

| Power Start [MW] | Power End [MW] | Incremental Heat Rate [MMBtu/MWh] | Fuel Use Rate [MMBtu/h] |
|---|---|---|---|
| $p_{g,1}^{\min}$ | . | . | $\gamma$ |
| $p_{g,1}^{\min}$ | $p_{g,1}^{\max}$ | $\delta_1$ | . |
| $p_{g,2}^{\min} = p_{g,1}^{\max}$ | $p_{g,2}^{\max}$ | $\delta_2$ | . |
| $p_{g,3}^{\min} = p_{g,2}^{\max}$ | $p_{g,3}^{\max}$ | $\delta_3$ | . |

Table 14: Input data example for fuel usage of a generation project.

In this case, the fuel use rate in the first row describes the fuel use rate at minimum load. However, the heat rate conversion will depend on the actual power generated. In order to ensure a convex boundary, it must hold that $\delta_3 \geq \delta_2 \geq \delta_1$. Literal dots must be included in the input files to indicate blanks. If no input data are provided for a project, then a single segment with a $y$-intercept of 0 and a slope equal to full load heat rate ($h_g$ from `generators.core.dispatch`) is used as the heat rate curve for that project.

### 4.3.16 transmission.local_td

This optional module defines model components to describe local transmission & distribution (T&D) build-outs for the Switch model. This adds a virtual "distribution node" to each load zone that is connected to the zone's central node via a distribution pathway that incurs distribution losses. Distributed Energy Resources (DER) impact the energy balance at the distribution node, potentially reducing losses from the distribution network and investments in distribution capacity.

For this purpose two sets (defined as Python lists) are created to account for the power injections $\mathcal{D}^{\text{inject}}$ and power withdrawals $\mathcal{D}^{\text{withdraw}}$ inside the distribution node.

If this module is used, the load zone demand $l_{z,t}$ will be added to the list $\mathcal{D}^{\text{withdraw}}$ instead of the list of the power grid withdrawal $\mathcal{P}^{\text{withdraw}}$ (it is assumed that the demand is inside the distribution node).

Table 15 presents the sets, parameters and variables used on this module:

| Type | Symbol | Description |
|---|---|---|
| Subset | $\mathcal{Z}^{\text{td}}$ | Subset of load zones where local T&D will be modeled. |
| Parameter | $b_z^{\text{td}}$ | Preexisting capacity for local T&D in load zone $z$ at the initial period (MW). |
| Variable | $B_{z,p}^{\text{td}}$ | Additions to local T&D capacity in zone $z$ at period $p$ (MW). |
| Variable | $K_{z,p}^{\text{td}}$ | Cumulative local T&D capacity in zone $z$ at period $p$. |
| Variable | $P_{z,t}^{\text{td,w}}$ | Power withdrawn in MW from a zone's central node that is going to be sent to its local T&D node. |
| Variable | $P_{z,t}^{\text{inj,i}}$ | Power injected in MW to the local T&D node. |
| Parameter | $\eta_z^{\text{td}}$ | Proportion of energy that is lost in local T&D system before delivery. |
| Parameter | $c_z^{\text{td}}$ | Annualized capital costs (includes fixed O&M costs) per MW for existing and new local infrastructure. |

Table 15: Model components defined in the `transmission.local_td` module.

The variables $P_{z,t}^{\text{td,w}}$ are added as power withdrawal components for the load zones and therefore added to the set $\mathcal{P}^{\text{withdraw}}$, while the variables $P_{z,t}^{\text{inj,i}}$ are added as power injections components for the distribution nodes and so added to the list $\mathcal{D}^{\text{inject}}$.

Each period, the system is required to have sufficient capacity to meet the local T&D requirements. For this purpose a constraint is added to satisfy the local maximum expected demand if the expected peak demand is specified:

$$K_{z,p}^{\text{td}} \geq \frac{l_{z,p}^{\text{peak}}}{1-\eta_z^{\text{td}}} \qquad \forall z \in \mathcal{Z}^{\text{td}}, \forall p \in \mathcal{P} \tag{46}$$

In addition, during every time period the power withdrawal from the main transmission node must not exceed the local T&D capacity:

$$P_{z,t}^{\text{td,w}} \leq K_{z,t}^{\text{td}}, \qquad \forall z \in \mathcal{Z}^{\text{td}}, \forall t \in \mathcal{T} \tag{47}$$

The cumulative capacity $K_{z,p}^{\text{td}}$ is calculated as:

$$K_{z,p}^{\text{td}} = b_z^{\text{td}} + \sum_{p' \in \mathcal{P}:\ p' \leq p} B_{z,p'}^{\text{td}}, \qquad \forall z \in \mathcal{Z}^{\text{td}}, \forall p \in \mathcal{P} \tag{48}$$

The relationship between the withdrawal from the central node and the injection to the distribution node is given by:

$$P_{z,t}^{\text{td,i}} = P_{z,t}^{\text{td,w}}(1 - \eta_z^{\text{td}}), \qquad \forall z \in \mathcal{Z}^{\text{td}}, \forall t \in \mathcal{T} \tag{49}$$

A dynamic equation must be considered in order to balance the power inside the distribution node:

$$\sum_{p^{\text{td,i}} \in \mathcal{D}^{\text{inject}}} p_{z,t}^{\text{td,i}} = \sum_{p^{\text{td,w}} \in \mathcal{D}^{\text{withdraw}}} p_{z,t}^{\text{td,w}}, \qquad \forall z \in \mathcal{Z}^{\text{td}}, \forall t \in \mathcal{T} \tag{50}$$

Finally the annualized cost of investment $c_z^{\text{td}} K_{z,p}^{\text{td}}$ is added as a cost component in the set $\mathcal{C}^{\text{fixed}}$ in order to be considered in the objective function (15).

This formulation allows users to create modules that include distributed energy resources. These modules will reduce the withdrawal from the central grid, since those components inject power only inside the distribution node. For now, this module does not allow backfeeding power from the distribution node to the central grid.

#### 4.3.17 balancing.demand_response.simple

This optional module describes a simple Demand Response (DR) load-shifting service. Load in each load zone may be shifted between time points belonging to the same timeseries at no cost. This allows assessing the potential value of demand shifting. Table 16 presents the parameters and variables defined in this module:

| Type | Symbol | Description |
|---|---|---|
| Parameter | $l_{z,t}^{\text{max,up}}$ | Maximum increase in demand allowed in load zone $z$ at time point $t$. |
| Parameter | $l_{z,t}^{\text{max,down}}$ | Maximum reduction in demand allowed in load zone $z$ at time point $t$. This value must be less than the local demand. |
| Variable | $L_{z,t}^{\text{dr}}$ | Describes how much load (in MW) is reduced (if it is negative) or increased (if it is positive) in load zone $z$ at timepoint $t$. |

Table 16: Model components defined in the `balancing.demand_response.simple` module.

The DR shift is bounded by the specified limits, and another constraint ensures that all the changes in demand balance out over the course of each timeseries:

$$-l_{z,t}^{\text{max,down}} \leq L_{z,t}^{\text{dr}} \leq l_{z,t}^{\text{max,up}}, \qquad \forall z \in \mathcal{Z}, \forall t \in \mathcal{T} \tag{51}$$

$$\sum_{t \in \mathcal{T}_s} L_{z,t}^{\text{dr}} = 0, \qquad \forall z \in \mathcal{Z}, \forall s \in \mathcal{S} \tag{52}$$

The demand shift $L_{z,t}^{\text{dr}}$ is added to the set $\mathcal{P}^{\text{withdraw}}$ in order to be included in the balance equation (16). If `transmission.local_td` is used, the demand shift is added to the distributed set $\mathcal{D}^{\text{withdraw}}$ instead.

#### 4.3.18 generators.extensions.hydro_simple

This optional module defines a simple hydro electric model that can be used to model dispatchable reservoir-based hydro plants with minimum and average water dispatch targets

that may vary by time point. A more complex hydro system is defined in the module `generators.extensions.hydro_system`, which includes an underlying water network, rainfall and ground infiltration. Table 17 presents the sets, parameters and variables defined in this module:

| Type | Symbol | Description |
|---|---|---|
| Subset | $\mathcal{G}^{\mathrm{H}}$ | Subset of all hydro-based generation projects. |
| Parameter | $p_{g,s}^{\mathrm{h,min}}$ | Minimum flow level, expressed as electrical MW, for all timepoints of timeseries $s$. |
| Parameter | $p_{g,s}^{\mathrm{h,avg}}$ | Average flow level, in electrical MW, that must be achieved during timeseries $s$. |

Table 17: Model components defined in the `generators.extensions.hydro_simple` module.

In this simple formulation, power dispatch must exceed the minimum level at all times, and the average power production during a time series must be equal to the specified average flow rate:

$$P_{g,t} \geq p_{g,s}^{\mathrm{h,min}}, \qquad \forall g \in \mathcal{G}^{\mathrm{H}}, \forall s \in \mathcal{S}, \forall t \in \mathcal{T}_s. \tag{53}$$

$$\frac{1}{\mathrm{num}_s} \cdot \sum_{t \in \mathcal{T}_s} P_{g,t} = p_{g,s}^{\mathrm{h,avg}}, \qquad \forall g \in \mathcal{G}^{\mathrm{H}}, \forall s \in \mathcal{S}. \tag{54}$$

#### 4.3.19 generators.extensions.hydro_system

This optional module creates a hydraulic system that works in parallel with the electric one. They are linked through the power generation process at hydro-based generators. It is required to define the specification of the water network topology, such as water nodes, reservoirs, water connections and hydroelectric generation projects. This module is mutually exclusive the `generators.extensions.hydro_simple` module.

The water network is a graph composed of nodes and connections. Nodes represent rivers, lakes or reservoirs, while connections represents water flows between nodes where generating stations may be located.

All nodes can have inflows and consumption that are independent of the electrical network. All connections can control flow between nodes, potentially limited by minimum flow constraints, or dictated by geological filtration. All flow is currently downstream, sink nodes have the ability to spill outside of the hydraulic system and reservoir nodes track their water levels during investment periods, and have their levels externally determined at the beginning and end of investment periods.

Table 18 presents the sets, parameters and variables defined in this module:

| Type | Symbol | Description |
|---|---|---|
| Subset | $\mathcal{G}^{\mathrm{H}}$ | Subset of all hydro-based generation projects. |
| Set | $\mathcal{N}$ | Set of nodes of the water system, indexed by $n$. |
| Subset | $\mathcal{N}^{\mathrm{R}}$ | Subset of water nodes that are reservoirs. |
| Subset | $\mathcal{N}^{\mathrm{S}}$ | Subset of water nodes that are sinks. |
| Set | $\mathcal{C}$ | Set of connections in the water network, indexed by $k$. |
| Subset | $\mathcal{C}_n^{\mathrm{in}}$ | Subset of connections directed into water node $n$. |
| Subset | $\mathcal{C}_n^{\mathrm{out}}$ | Subset of connections directed out of water node $n$. |
| Subset | $\mathcal{G}_k^{\mathrm{H}}$ | Subset of hydro-based generation located in connection $k$. |
| Parameter | $w_{n,t}$ | Natural water inflow in node $n$ at time point $t$. |
| Parameter | $l_{n,t}^{\mathrm{h}}$ | Water consumption, not related to electric generation, in node $n$ at time point $t$. |
| Variable | $S_{nt}$ | Water spillage out of the water network in node $n$ at time point $t$ in $\mathrm{m}^3$/s. |
| Parameter | $c^{\mathrm{spill}}$ | Cost in \$/$\mathrm{m}^3$ of spilling water out of the water network. |
| Parameter | $v_{n,t}^{\min} \in \mathcal{N}^{\mathrm{R}}$ | Minimum storage capacity in millions of $\mathrm{m}^3$ of reservoir $n$ at time point $t$. |
| Parameter | $v_{n,t}^{\max} \in \mathcal{N}^{\mathrm{R}}$ | Maximum storage capacity in millions of $\mathrm{m}^3$ of reservoir $n$ at time point $t$. |
| Parameter | $v_n^{\mathrm{init}} \in \mathcal{N}^{\mathrm{R}}$ | Volume of stored water in millions of $\mathrm{m}^3$ at the beginning of each period of reservoir $n$. |
| Parameter | $v_n^{\mathrm{end}} \in \mathcal{N}^{\mathrm{R}}$ | Volume of stored water in millions of $\mathrm{m}^3$ at the end of each period of reservoir $n$. |
| Variable | $V_{n,t}^{\mathrm{hydro}}$ | Volume of stored water in units of $\mathrm{m}^3$ in node $n$ at time point $t$. It will be different than zero only in reservoir nodes. |
| Variable | $W_{k,t}^{\mathrm{hydro}}$ | Water flow through connection $k$ at time point $t$. |
| Parameter | $w_{n,t}^{\min}$ | Minimum ecological water flow that must be dispatched through connection $k$ at time point $t$, in $\mathrm{m}^3$/s. |
| Parameter | $w_{n,t}^{\max}$ | Maximum water flow that can be dispatched through connection $c$ at time point $t$, in $\mathrm{m}^3$/s. |
| Parameter | $\eta_g^{\mathrm{h}} \in \mathcal{G}^{\mathrm{H}}$ | Hydraulic efficiency of project $g$ in MW/($\mathrm{m}^3$/s). |

Table 18: Model components defined in the `generators.extensions.hydro_system` module.

This formulation adds several constraints to the model:

$$w_{n,t} + \sum_{c \in \mathcal{C}_n^{\mathrm{in}}} W_{k,t}^{\mathrm{hydro}} + V_{n,t}^{\mathrm{hydro}} = \sum_{c \in \mathcal{C}_n^{\mathrm{out}}} W_{k,h}^{\mathrm{hydro}} + V_{n,t+1}^{\mathrm{hydro}} \qquad \forall n \in \mathcal{N}, \forall t \in \mathcal{T} \tag{55}$$

$$v_{n,t}^{\min} \leq V_{n,t}^{\mathrm{hydro}} \leq v_{n,t}^{\max}, \qquad n \in \mathcal{N}^{\mathrm{R}}, \forall t \in \mathcal{T} \tag{56}$$

$$V_{n,t}^{\mathrm{hydro}} = v_n^{\mathrm{init}}, \qquad \forall n \in \mathcal{N}^{\mathrm{R}}, t = \mathrm{first}(\mathcal{T}_p), \forall p \in \mathcal{P} \tag{57}$$

$$V_{n,t}^{\mathrm{hydro}} \geq v_n^{\mathrm{end}}, \qquad \forall n \in \mathcal{N}^{\mathrm{R}}, t = \mathrm{last}(\mathcal{T}_p), \forall p \in \mathcal{P} \tag{58}$$

$$\frac{P_{g,t}}{\eta_g^{\mathrm{h}}} + S_{g,t} = W_{k,t}^{\mathrm{hydro}}, \qquad \forall g \in \mathcal{G}_k^{\mathrm{H}}, \forall k \in \mathcal{C}, \forall t \in \mathcal{T}. \tag{59}$$

Constraint (55) ensures the conservation of mass at each node and time point. Equation (56) bound the storage of reservoirs, while equations (57) and (58) are the boundary conditions for the reservoirs at each period. Equation (59) links the water network to the hydro-based generators, where water flows are used to produce electricity. Multiple projects may be located at the same connection, which allows modeling of cascading generation.

Finally, the spillage costs $c^{\mathrm{spill}} S_{g,t}$ are added to the set $\mathcal{C}^{\mathrm{var}}$ in order to be considered in the objective function (15).

Figure 3 illustrates some networks that have been modeled using this module.

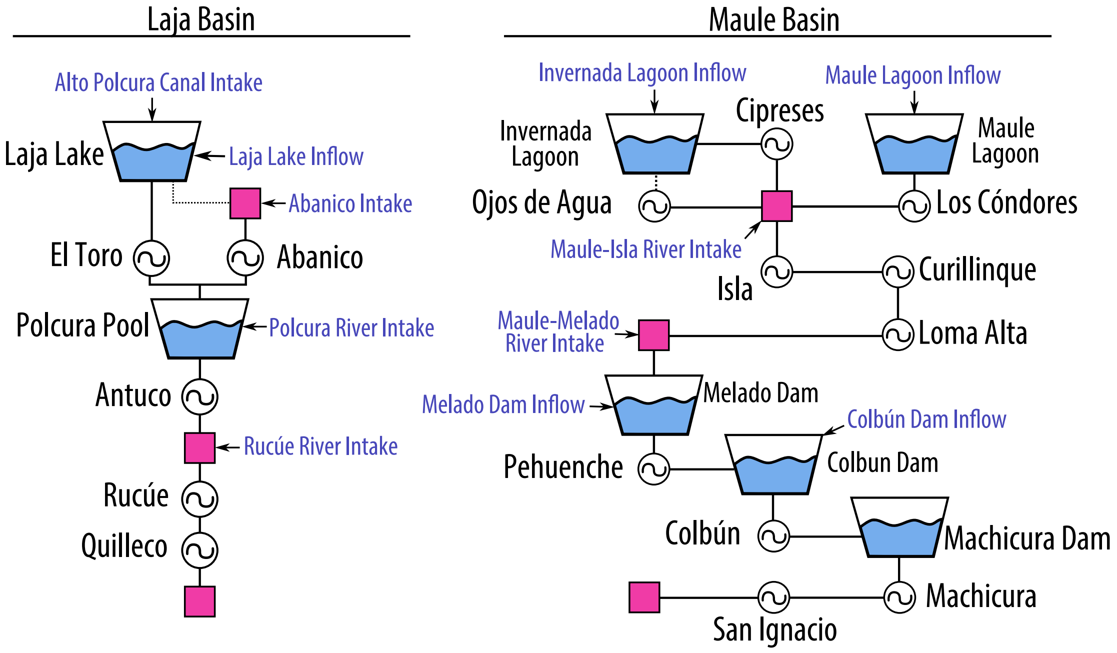


Figure 3: Two hydraulic basins of Chile with hydroelectric generators.

#### 4.3.20 generators.extensions.storage

This optional module defines generic storage technologies. It extends the generic generator model, adding components to decide how much energy-storage capacity to build in each project (in addition to the standard power-throughput capacity) and when to charge storage, and to account for energy levels over time. Table 19 presents the sets, parameters and variables defined in this module.

| Type | Symbol | Description |
|---|---|---|
| Subset | $\mathcal{G}^{\text{S}}$ | Subset of all generation projects that can store electricity for later discharge. |
| Parameter | $\eta_g^{\text{S}}$ | Round trip efficiency of a storage technology. Self-discharge over time is assumed to be negligible. |
| Parameter | $\hat{c}_{g,p}^{\text{S,inv}}$ | Overnight capital cost per MWh adding energy storage capacity (not power output) to storage project $g$ in period $p$. |
| Parameter | $r_g^{\text{max}}$ | The maximum charging rate for storage project $g$, expressed as a ratio relative to the maximum power output rate. |
| Parameter | $b_{g,p}^{\text{S}}$ | Predetermined installed energy capacity of project $g$ at period $p$. |
| Subset | $\mathcal{P}_g^{\text{S}}$ | Subset of periods in which the investment of storage project $g$ is predetermined (may include periods in the past). |
| Variable | $B_{g,p}^{\text{S}}$ | Amount of energy storage capacity to add to project $g \in \mathcal{G}^{\text{S}}$ in period $p$, in MWh. |
| Variable | $K_{g,p}^{\text{S}}$ | Cumulative capacity in MWh of storage project $g$ at period $p$. |
| Variable | $C_{g,t}^{\text{S}}$ | Decision of how much to charge a storage project $g$ at time point $t$. |
| Variable | $P_{g,t}$ | Decision of how much to discharge a storage project $g$ at time point $t$, i.e., how much power to deliver to the grid (defined in `generators.core.build`). |
| Variable | $\overline{P_{g,t}}$ | Maximum possible power production by project $g$ at timepoint $t$, (defined by equation (34) or (39)). |
| Variable | $Z_{g,t}^{\text{S}}$ | State of charge in MWh of storage project $g$ at timepoint $t$. |

Table 19: Model components defined in the `generators.extensions.storage` module.

Overnight costs $\hat{c}^{\text{S,inv}}_{g,p}$ are annualized, and then these costs $c^{S,\text{inv}}_{g,p}B^S_{g,p}$ are added to the set $\mathcal{C}^{\text{fixed}}$ in order to be considered in the objective function (15).

Power used for charging is added to the set of withdrawals $\mathcal{P}^{\text{withdraw}}$ for inclusion in the balance equation (16). Power produced by discharging storage is already added to $\mathcal{P}^{\text{inject}}$ by `generators.core.build`.

This formulation defines several constraints to restrict the use of storage systems and account for the ongoing energy balance:

$$K^{\text{S}}_{g,p} = \sum_{p' \in \mathcal{P}:\ p' \leq p} B^{\text{S}}_{g,p'}, \qquad \forall g \in \mathcal{G}^{\text{S}}, p \in \mathcal{P} \tag{60}$$

$$B_{g,p} = b^{\text{S}}_{g,p}, \qquad \forall g \in \mathcal{G}^{\text{S}}, p \in \mathcal{P}^{\text{S}}_g \tag{61}$$

$$0 \leq C^{\text{S}}_{g,t} \leq r^{\max}_g \overline{P_{g,t}}, \qquad \forall g \in \mathcal{G}^{\text{S}}, t \in \mathcal{T}^{\text{on}}_g \tag{62}$$

$$0 \leq Z^{\text{S}}_{g,t} \leq K^{\text{S}}_{g,p}, \qquad \forall g \in \mathcal{G}^{\text{S}}, t \in \mathcal{T}^{\text{on}}_g \tag{63}$$

$$Z^{\text{S}}_{g,t} = Z^{\text{S}}_{g,t-1} + (\eta^{\text{S}}_g C^{\text{S}}_{g,t} - P_{g,t})\Delta_{s(t)}, \qquad \forall g \in \mathcal{G}^{\text{S}}, t \in \mathcal{T}^{\text{on}}_g \tag{64}$$

Equation (60) defines the cumulative energy storage capacity by the sum of the previous investments. Equation (61) models predetermined investment in some periods, such as installed capacity before the initial period. Equations (62) and (63) limit the charging capacity and state of charge depending on the installed capacity. Finally, equation (64) tracks the evolution of the state of charge of each project, depending on the rate of charging and discharging at each timepoint.

### 4.3.21 policies.rps_simple

This optional module defines a simple Renewable Portfolio Standard (RPS) policy scheme for the Switch model. In this scheme, each fuel is characterized as RPS-eligible or not. All non-fuel energy sources are assumed to be RPS-elegible. Electricity that is generated from RPS-elegible sources in each period is summed up and must meet an energy goal, set as a required percentage of the total demand in that period. This module only works with the `no_commit` package. The Hawaii regional subpackage contains a more advanced RPS module that works with unit commitment and considers multi-fuel generators.

Table 20 presents the sets, parameters and variables defined in this module:

| Type | Symbol | Description |
|---|---|---|
| Subset | $\mathcal{G}^{\text{RPS}}$ | Subset of all generators that are RPS eligible. |
| Parameter | $\text{rps}_p$ | Fraction of total demand in period $p$ that must be generated from RPS-elegible sources. |

Table 20: Model components defined in the `policies.rps_simple` module.

The RPS target in each period is enforced via the following constraint:

$$\sum_{t \in \mathcal{T}_p} \sum_{g \in \mathcal{G}^{\text{RPS}}} P_{g,t} \geq \text{rps}_p \times \sum_{t \in \mathcal{T}_p} \sum_{z \in \mathcal{Z}} l_{z,t}, \qquad \forall p \in \mathcal{P} \tag{65}$$

#### 4.3.22 policies.carbon_policies

This optional module adds carbon emission policies to the model, either in the form of emission caps or in the form of a cost adder that could represent the social cost of carbon, a carbon tax, or the expected clearing price of a cap-and-trade carbon market.

Table 21 presents the parameters defined in this module:

| Type | Symbol | Description |
|---|---|---|
| Parameter | $\text{cap}_p$ | Carbon cap in tons of $CO_2$ per year during period $p$ (defaults to $\infty$). |
| Parameter | $c_p^{\text{carb}}$ | Carbon cost per ton of $CO_2$ in period $p$ (defaults to \$0). |

Table 21: Model components defined in the `policies.carbon_policies` module.

The systemwide annual emission rate of $CO_2$ is calculated (in `generators.core.dispatch`) as

$$\text{AnnualEmissions}_p = \sum_{g \in \mathcal{G}^{\text{F}}} \sum_{f \in \mathcal{E}_g^{\text{F}}} \sum_{t \in \mathcal{T}_g^{on} \cap \mathcal{T}_p} \Delta_{s(t)} R_{g,t,f} \times (\xi_f + \mu_f), \qquad \forall p \in \mathcal{P} \tag{66}$$

To model carbon costs, the term:

$$c_p^{\text{carb}} \cdot \text{AnnualEmissions}_p$$

is added to the set $\mathcal{C}^{\text{fixed}}$ for inclusion in the objective function (15).

A carbon cap is modeled via the constraint:

$$\text{AnnualEmissions}_p \leq \text{cap}_p, \qquad \forall p \in \mathcal{P}. \tag{67}$$

#### 4.3.23 balancing.unserved_load

This optional module relaxes the load-serving constraints, allowing some load to be left unserved, with a penalty. This module is especially useful for ensuring feasibility and identifying shortfalls when running production costing simulations. Table 22 presents the parameters and variables defined in this module:

| Type | Symbol | Description |
|---|---|---|
| Variable | $X_{z,t}$ | Decision of how much load in MWh is not supplied in zone $z$ at timepoint $t$. |
| Parameter | $c^{\text{pen}}$ | Penalty charge per MWh for leaving load unserved. |

Table 22: Model components defined in the `balancing.unserved_load` module.

The penalty cost of not supplying load $c^{\text{pen}} X_{z,t}$ is added to the set $\mathcal{C}^{\text{var}}$ in order to be considered in the objective function (15). The unserved load $X_{z,t}$ is added to the set $\mathcal{P}^{\text{inject}}$ in order to be considered in the power balance equation (16).

Users should set the penalty $c^{\text{pen}}$ to a high value relative to the cost of generation, and should inspect the unserved load variable $X_{z,t}$ to identify any shortfalls in their system design.

#### 4.3.24 balancing.planning_reserves

This optional module defines planning reserves requirements ($\pi$) to support resource adequacy requirements. These requirements are sometimes called capacity reserve margins. The general idea is that if a system has a percentage of generation capacity above and beyond demand, then the grid can maintain adequate reliability.

Table 23 presents the sets and parameters defined in this module:

| Type | Symbol | Description |
|---|---|---|
| Set | $\Pi$ | Set of planning reserve requirements to be enforced. Each requirement applies to a particular collection of load zones and timepoints. Indexed by $\pi$. |
| Subset | $\mathcal{Z}_\pi^{\mathrm{PR}}$ | Subset of load zones that are considered when enforcing PRR $\pi$. |
| Subset | $\mathcal{T}_\pi^{\mathrm{PR}}$ | Subset of timepoints when PRR $\pi$ has effect. Each PRR $\pi$ may apply to all timepoints, or just the timepoint with the expected peak load demand. |
| Subset | $\mathcal{G}_\pi^{\mathrm{PR}}$ | Subset of generators that are considered to provide capacity reserves for PRR $\pi$. |
| Parameter | $\kappa_\pi$ | Capacity reserve margin for each PRR $\pi$ (defaults to 0.15). |
| Parameter | $\kappa_{g,t}^{\mathrm{gen}}$ | How much of a generator's installed capacity is credited towards $\pi$ at time point $t$. This parameter defaults to $\eta_{g,t}$ for renewable projects, and 1.0 to other plants. |

Table 23: Model components defined in the `balancing.planning_reserves` module.

This module also defines two dynamic sets of components (implemented as Python lists of Pyomo model objects):

- Available capacity for reserves $\mathcal{R}^{\mathrm{cap}}$: set of components $r^{\mathrm{c}}$ that contribute to satisfying planning reserve requirements. Each component in this list should be indexed by requirement $\pi$ and timepoint $t$, and specified in units of MW.
- Requirements for capacity reserves $\mathcal{R}^{\mathrm{req}}$: set of components $r^{\mathrm{r}}$ that contribute to planning reserve requirements. Each component in this list should be indexed by requirement $\pi$ and timepoint $t$, and specified in units of MW.

This module adds terms a number of terms to the dynamic sets of planning reserve components. Thus, several elements are added to the sets $\mathcal{R}^{\mathrm{cap}}$ and $\mathcal{R}^{\mathrm{req}}$:

- Generation and storage technologies: Generators are credited based on their installed capacity, but storage is credited based on its expected output (net of charging) at the specific timepoint considered. The term

$$\sum_{g \in \mathcal{G}_\pi^{\mathrm{PR}} - \mathcal{G}^{\mathrm{S}}} \kappa_{g,t}^{\mathrm{gen}} K_{g,p(t)} + \sum_{g \in \mathcal{G}_\pi^{\mathrm{PR}} \cap \mathcal{G}^{\mathrm{S}}} \left( \kappa_{g,t}^{\mathrm{gen}} P_{g,t} - C_{g,t}^{\mathrm{S}} \right), \qquad \forall \pi \in \Pi, \forall t \in \mathcal{T}_\pi^{\mathrm{PR}}. \tag{68}$$

  is added to $\mathcal{R}^{\mathrm{cap}}$ as available capacity for planning reserves.

- Transmission flows: Like storage, transmission lines are credited toward capacity planning based on their expected use during the relevant timepoints. The term

$$\sum_{z \in \mathcal{Z}_\pi^{PR}} \sum_{\ell \in \mathcal{L}_z^{in}} F_{\ell,t}, \qquad \forall \pi \in \Pi, \forall t \in \mathcal{T}_\pi^{\mathrm{PR}} \tag{69}$$

  is added to $\mathcal{R}^{\mathrm{cap}}$ as available capacity for reserves.

- Demand requirements: The term

$$(1 + \kappa_\pi) \sum_{z \in \mathcal{Z}_\pi^{PR}} l_{z,t}, \qquad \forall \pi \in \Pi, \forall t \in \mathcal{T}_\pi^{\mathrm{PR}} \tag{70}$$

is added to $\mathcal{R}^{\mathrm{req}}$ as a requirement for capacity reserves.

Finally constraints representing the planning reserve requirements are constructed dynamically as:

$$\sum_{r^{\mathrm{c}} \in \mathcal{R}^{\mathrm{cap}}} r^{\mathrm{c}}_{\pi,t} \quad \geq \sum_{r^{\mathrm{r}} \in \mathcal{R}^{\mathrm{req}}} r^{\mathrm{r}}_{\pi,t}, \qquad \forall \pi \in \Pi, \forall t \in \mathcal{T}_\pi^{\mathrm{PR}} \tag{71}$$

where the term $r^{\mathrm{c}}$ indicates a Pyomo component that has been placed in the set $\mathcal{R}^{\mathrm{cap}}$ (e.g., the expressions defined in (68) and (69)), and $r^{\mathrm{c}}_{\pi,t}$ indicates the element of $r^{\mathrm{c}}$ with indexes $(\pi, t)$. A similar definition holds for the reserve requirements terms $r^{\mathrm{r}}_{\pi,t}$.

#### 4.3.25 balancing.operating_reserves.areas

This module defines the balancing areas where operating reserve requirements will be applied. Table 24 presents the sets and parameters defined in this module.

| Type | Symbol | Description |
|---|---|---|
| Set | $\mathcal{B}$ | Set of balancing areas where operating reserve requirements will be enforced, indexed by $b$. Each balancing area spans one or more load zones. |
| Subset | $\mathcal{Z}_b^{\mathrm{bal}}$ | Subset of load zones in balancing area $b$. |

Table 24: Model components defined in the `balancing.operating_reserves.areas` module.

#### 4.3.26 balancing.operating_reserves.spinning_reserves

This module defines a flexible framework for considering spinning reserve requirements. Most regions have their own rules for defining spinning reserve requirements, so we provide a framework for specifying custom requirements along with two examples of concrete requirements. This module requires the `generators.core.commit.operate` package to be used. Several dynamic sets (defined as Python lists) are created to allow other modules to register their effect on reserve requirements:

- Available spinning reserves for satisfying up and down reserve requirements: $\mathcal{S}^{\mathrm{u,res}}$ and $\mathcal{S}^{\mathrm{d,res}}$ are sets of components, $s^{\mathrm{u,res}}$ and $s^{\mathrm{d,res}}$, that contribute to satisfy spinning reserve requirements. Each component in these sets needs to be indexed by balancing area $b$ and time point $t$, and specified in units of MW.

- Requirements for upward and downward spinning reserves: $\mathcal{S}^{\mathrm{u,req}}$ and $\mathcal{S}^{\mathrm{d,req}}$ are sets of components $s^{\mathrm{u,req}}$ and $s^{\mathrm{d,req}}$ that define or increase spinning reserve requirements. Each component in these sets needs to be indexed by balancing area $b$ and time point $t$, and specified in units of MW.

- Spinning reserves contingencies: $\mathcal{S}^{\mathrm{u,cont}}$ is a set of components that define possible upward contingency events (loss of generation). Each component in this set should be a Pyomo object

indexed by balancing area $b$, and timepoint $t$, and specified in units of MW, identifying a contingency that could occur at that place and time. As described below, the system will maintain additional spinning reserves to compensate for the largest contingency in each balancing area during each timepoint.

Table 25 presents the other sets, variables and parameters defined in this module:

| Type | Symbol | Description |
|---|---|---|
| Set | $\mathcal{G}^{\text{spin}}$ | Set of generators that can provide spinning reserves. |
| Subset | $\mathcal{G}_b^{\text{B}}$ | Subset of generators that are located in balancing zone $b$. |
| Parameter | sf | "Safety factor" parameter that increases the contingency reserve requirement. By default this is set to 1.0, providing just enough reserves for the single largest contingency. |
| Variable | $S_{g,t}^{\text{up}}$ | Amount of upward spinning reserves to provide from generator $g$ in timepoint $t$ (MW). |
| Variable | $S_{g,t}^{\text{down}}$ | Amount of downward spinning reserves to provide from generator $g$ in timepoint $t$ (MW). |

Table 25: Model components defined in the `balancing.operating_reserves.spinning_reserves` module.

Limits on upward and downward spinning reserves are imposed based on the available capacity:

$$S_{g,t}^{\text{up}} \leq \eta_{g,t} K_{g,p(t)}^{\text{G}} - W_{g,t}, \qquad \forall g \in \mathcal{G}^{\text{spin}}, \forall t \in \mathcal{T} \tag{72}$$

$$S_{g,t}^{\text{down}} \leq W_{g,t}, \qquad \forall g \in \mathcal{G}^{\text{spin}}, \forall t \in \mathcal{T} \tag{73}$$

The terms:

$$\sum_{g \in \mathcal{G}^{\text{spin}} \cap \mathcal{G}_b^{\text{B}}} S_{g,t}^{\text{up}}, \qquad \forall b \in \mathcal{B}, \forall t \in \mathcal{T}$$

$$\sum_{g \in \mathcal{G}^{\text{spin}} \cap \mathcal{G}_b^{\text{B}}} S_{g,t}^{\text{down}}, \qquad \forall b \in \mathcal{B}, \forall t \in \mathcal{T}$$

are added to the available spinning reserves for satisfying up $\mathcal{S}^{\text{u,res}}$ and down $\mathcal{S}^{\text{d,res}}$ requirements, respectively.

This module includes some example rules for setting regulating reserve requirements, which can be used as-is by specifying a command-line argument, or copied as a starting point for a custom module.

One example rule, "3+5" is based on a heuristic, described in NREL's 2010 Western Wind and Solar Integration study, that requires spinning reserves (both up and down) of 3% of load plus 5% of renewable output. The "3+5" regulating reserve requirements are calculated as:

$$0.03 \sum_{z \in \mathcal{Z}_b^{\text{bal}}} l_{z,t} + 0.05 \sum_{g \in \mathcal{G}^{\text{R}} \cap \mathcal{G}_b^{\text{B}}} P_{g,t}, \qquad \forall b \in \mathcal{B}, \forall t \in \mathcal{T}$$

and added to the spinning reserve requirement sets for both up $\mathcal{S}^{\text{u,req}}$ and down $\mathcal{S}^{\text{d,req}}$ reserves.

The other example rule, "Hawaii" is based on reserve rules developed by General Electric Energy Consulting (GE) for the Hawaii Renewable Portfolio Standards Study (RPS Study, `https://www.hnei.hawaii.edu/projects/hawaii-rps-study`). In the RPS Study, GE estimated the

amount of regulating reserves that would be adequate to compensate for forecast errors for 18 different portfolios of wind and solar power, as a function of the amount of renewable power available each hour. Regression analysis indicated that these reserves could be fit well by assigning 100% reserves for the available wind and solar power up to a limit of 21.6% or 21.3% of the installed capacity, respectively. (GE found forecast errors did not grow as production went above this level, so additional reserves were not needed for windier or sunnier hours). Based on these findings, the "Hawaii" regulating reserve requirements are calculated as:

$$\sum_{g \in \mathcal{G}_b^{\mathrm{B}}} K_{g,p(t)}^{\mathrm{G}} \times \min \left\{ \begin{array}{l} \eta_{g,t}, \\ \left\{ \begin{array}{l} 0.216 \text{ if } \mathcal{E}_g^{\mathrm{F}} = \{\text{wind}\}, \\ 0.213 \text{ if } \mathcal{E}_g^{\mathrm{F}} = \{\text{sun}\}, \\ 0.000 \text{ otherwise} \end{array} \right\} \end{array} \right\}, \qquad \forall t \in \mathcal{T}, b \in \mathcal{B}$$

and added to the upward spinning reserve requirement set, $\mathcal{S}^{\mathrm{u,req}}$.

The "Hawaii" rule also allocates down reserves equal to 10% of loads during each timepoint, matching the treatment in the RPS Study. This is implemented by calculating the following term:

$$\sum_{z \in \mathcal{Z}_b^{\mathrm{bal}}} 0.1 \; l_{z,t} \qquad \forall t \in \mathcal{T}, b \in \mathcal{B}$$

and adding it to the downward spinning reserve requirement set, $\mathcal{S}^{\mathrm{d,req}}$

This module also offers two strategies for calculating contingency reserve requirements, selectable via command-line options. The first strategy enables $n-1$ contingency reserves based on the largest single unit of any generation project tripping offline. This creates a new binary variable for each timepoint for each project that has a discrete unit size $b_g^{\mathrm{unit}}$ specified (see `generators.core.build`). The second strategy defines $n-1$ contingencies based on the entire committed capacity of a generation project tripping offline. Unlike the first strategy, this is a continuous, linear expression. The second strategy is most suitable for studies where each project represents a single generating unit. The following subsubsections describe how each type of contingency is modeled.

#### 4.3.26.1 Unit-based contingency

This section describes components that are used to identify the largest unit-level contingency that could occur in each timepoint, if the user selects the unit-based contingency option. This models contingencies of individual generation units that have discrete sizes specified $\mathcal{G}^{\mathrm{unit}}$ (typically thermal plants and possibly large, single-contingency renewable facilities). This approach adds binary variables to the model for each timepoint for each discrete-sized project. Table 26 presents the variables defined if this option is selected:

| Type | Symbol | Description |
|---|---|---|
| Variable | $W_{g,t}^{\text{commit}}$ | Binary variable $\{0,1\}$ that indicates whether at least one unit is committed in generation project $g$ in timepoint $t$. |
| Variable | $P_{b,t}^{\text{cont}}$ | Variable that is constrained to show the size of the largest contingency in balancing area $b$ during timepoint $t$, accounting for all discretely sized units that are committed at that time. |

Table 26: Additional model components defined in `balancing.operating_reserves.spinning_reserves` module when using the unit-based contingency option.

Two constraints are defined for assessing the largest contingency:

$$W_{g,t} \leq m^{\text{big}} \cdot W_{g,t}^{\text{commit}}, \qquad \forall g \in \mathcal{G}^{\text{unit}}, \forall t \in \mathcal{T}_g^{\text{on}} \tag{74}$$

$$P_{b,t}^{\text{cont}} \geq W_{g,t}^{\text{commit}} \cdot b_g^{\text{unit}}, \qquad \forall b \in \mathcal{B}, \forall g \in \mathcal{G}^{\text{unit}} \cap \mathcal{G}_b^{\text{B}}, \forall t \in \mathcal{T}_g^{\text{on}} \tag{75}$$

Equation (74) uses a big M constraint with ($m^{\text{big}}$=100 GW by default) to force the $W_{g,t}^{\text{commit}}$ flag to be set to 1 for all projects that are committed, i.e., if $W_{g,t} > 0$. Equation (75) forces $P_{b,t}^{\text{cont}}$ to be greater than all the possible contingencies. Using this formulation, $P_{b,t}^{\text{cont}}$ must be set at least equal to the largest unit-based contingency. Finally, the $P^{\text{cont}}$ component is added to the set $\mathcal{S}^{\text{u,cont}}$ in order to be considered as a contingency.

#### 4.3.26.2 Project-based contingency

This section describes components that are used to identify the largest project-level contingency in each balancing area during each timepoint. These components are only added to the model if the user chooses this strategy via a command-line option. This approach maintains enough reserves to compensate for contingencies of entire generation projects tripping offline. For this purpose, a variable $P_{b,t}^{\text{p,cont}}$ is used to track the size of the largest project contingency in each balancing area by requiring:

$$P_{g,t}^{\text{p,cont}} \geq P_{g,t} + S_{g,t}^{\text{up}}, \qquad \forall b \in \mathcal{B}, \forall g \in \mathcal{G}_b^{\text{B}} \cap \mathcal{G}^{\text{spin}}, \forall t \in \mathcal{T}_g^{\text{on}} \tag{76}$$

$$P_{g,t}^{\text{p,cont}} \geq P_{g,t}, \qquad \forall b \in \mathcal{B}, \forall g \in \mathcal{G}_b^{\text{B}} \setminus \mathcal{G}^{\text{spin}}, \forall t \in \mathcal{T}_g^{\text{on}} \tag{77}$$

Equation (76) considers that the dispatch and available spinning up reserve can trip off for generators that are allowed to provide reserves, while equation (77) only considers the dispatch for generators that do not provide reserves. Finally, the $P^{\text{p,cont}}$ component is added to the set $\mathcal{S}^{\text{u,cont}}$ in order to be considered as a contingency.

#### 4.3.26.3 Dynamic reserve constraints

An additional variable $P_{b,t}^{\text{max,cont}}$ is defined to calculate the amount of spinning reserves that must be allocated to satisfy the system's contingency reserve requirement. $P_{b,t}^{\text{max,cont}}$ is set to an appropriate value by the constraint:

$$P_{b,t}^{\text{max,cont}} \geq \text{sf} \cdot s_{b,t}^{\text{u,cont}}, \qquad \forall b \in \mathcal{B}, \forall t \in \mathcal{T}, \forall s_{b,t}^{\text{u,cont}} \in \mathcal{S}^{\text{u,cont}} \tag{78}$$

Equation (78) ensures that $P_{b,t}^{\text{max,cont}}$ is greater than all the contingencies listed in $\mathcal{S}^{\text{u,cont}}$ multiplied by the security factor $sf$. The $\mathcal{S}^{\text{u,cont}}$ set may include the largest unit-level or project-level contingency in each balancing area, or other contingencies specified by the user. The contingency reserve requirement $P_{b,t}^{\text{max,cont}}$ is added to the system's set of upward spinning reserve requirements $\mathcal{S}^{\text{u,req}}$.

Finally, constraints are defined to satisfy the up and down spinning reserve requirements:

$$\sum_{s^{\text{u,res}} \in \mathcal{S}^{\text{u,res}}} s_{b,t}^{\text{u,res}} \geq \sum_{s^{\text{u,req}} \in \mathcal{S}^{\text{u,req}}} s_{b,t}^{\text{u,req}}, \qquad \forall b \in \mathcal{B}, \forall t \in \mathcal{T} \tag{79}$$

$$\sum_{s^{\text{d,res}} \in \mathcal{S}^{\text{d,res}}} s_{b,t}^{\text{d,res}} \geq \sum_{s^{\text{d,req}} \in \mathcal{S}^{\text{d,req}}} s_{b,t}^{\text{d,req}}, \qquad \forall b \in \mathcal{B}, \forall t \in \mathcal{T} \tag{80}$$

As with the objective function and energy balancing constraints, the $\mathcal{S}^{*,*}$ sets contain Pyomo components (expressions, variables or parameters) that are added to them at runtime by standard or custom modules. The $s^{*,*}$ variables refer to individual Pyomo components from these sets, and the $s_{b,t}^{*,*}$ terms refer to the element of $s^{*,*}$ with index $(b, t)$.

#### 4.3.27 balancing.operating_reserves.spinning_reserves_advanced

This module is an alternative to `balancing.operating_reserves.spinning_reserves` that allows the user to define requirements for multiple spinning reserve products. This can be used, for example, if some generation projects can supply both contingency and regulating reserves, but others can provide only contingency reserves, or if a power system defines separate fast-ramping and slow-ramping reserve requirements.

This module requires the `generators.core.commit.operate` package to be used. Several dynamic sets (defined as Python lists) are created to allow other modules to register their effect on reserve requirements:

- Available spinning reserves for satisfying up and down reserve requirements: $\mathcal{S}^{\text{u,res}}$ and $\mathcal{S}^{\text{d,res}}$ are sets of components, $s^{\text{u,res}}$ and $s^{\text{d,res}}$, that contribute to satisfy spinning reserve requirements. Each component in these sets must to be indexed by reserve type $r$, balancing area $b$ and time point $t$, and specified in units of MW. However, the components do not need to provide values for all possible combinations of these indexes; any missing values will be treated as 0. Note that this uses an additional indexing term $(r)$ that is not used in the simpler `balancing.operating_reserves.spinning_reserves` module.
- Requirements for upward and downward spinning reserves: $\mathcal{S}^{\text{u,req}}$ and $\mathcal{S}^{\text{d,req}}$ are sets of components $s^{\text{u,req}}$ and $s^{\text{d,req}}$ that define or increase spinning reserve requirements. Each component in these sets should be indexed by reserve type
- Spinning reserves contingencies: $\mathcal{S}^{\text{u,cont}}$ and $\mathcal{S}^{\text{d,cont}}$ are sets of components that define possible contingency events in the "up" (loss of generation) and "down" (loss of load) direction. (Note that the "down" direction is not included in the `balancing.operating_reserves.spinning_reserves` module.) Each component in these sets should be a Pyomo object indexed by balancing area $b$, and timepoint $t$, and specified in

units of MW, identifying a contingency that could occur at that place and time. As described below, the system will maintain additional spinning reserves to compensate for the largest contingency in each balancing area during each timepoint.

Table 27 presents the other sets, variables and parameters defined in this module:

| Type | Symbol | Description |
|---|---|---|
| Set | $\mathcal{G}^{\text{spin}}$ | Set of generators that can provide spinning reserves of any type. |
| Set | $\mathcal{R}_g^{\text{type}}$ | Set of spinning reserve types that can be provided by generation project $g \in \mathcal{G}^{\text{spin}}$. |
| Subset | $\mathcal{G}_b^{\text{B}}$ | Subset of generators that are located in balancing area $b$. |
| Parameter | sf | "Safety factor" parameter that increases the contingency reserve requirement. By default this is set to 1.0, providing just enough reserves for the single largest contingency. |
| Parameter | $r^{\text{reg}}$ | Type of reserve to use to meet regulation requirements (e.g., renewable power forecast errors). Defaults to "spinning" (generic spinning reserve product) |
| Parameter | $r^{\text{cont}}$ | Type of reserve to use to meet contingency requirements (e.g., loss of generation). Defaults to "spinning" (generic spinning reserve product). |
| Variable | $S_{r,g,t}^{\text{up}}$ | Amount of upward spinning reserves of type $r \in \mathcal{R}_g^{\text{type}}$ to provide from generator $g$ in timepoint $t$ (MW). |
| Variable | $S_{r,g,t}^{\text{down}}$ | Amount of downward spinning reserves of type $r \in \mathcal{R}_g^{\text{type}}$ to provide from generator $g$ in timepoint $t$ (MW). |

Table 27: Model components defined in the `balancing.operating_reserves.spinning_reserves_advanced` module.

Limits on upward and downward spinning reserves are imposed based on the available capacity:

$$\sum_{r \in \mathcal{R}_g^{\text{type}}} S_{r,g,t}^{\text{up}} \leq \eta_{g,t} K_{g,p(t)}^{\text{G}} - W_{g,t}, \qquad \forall g \in \mathcal{G}^{\text{spin}}, \forall t \in \mathcal{T} \tag{81}$$

$$\sum_{r \in \mathcal{R}_g^{\text{type}}} S_{r,g,t}^{\text{down}} \leq W_{g,t}, \qquad \forall g \in \mathcal{G}^{\text{spin}}, \forall t \in \mathcal{T} \tag{82}$$

The terms:

$$\sum_{g \in \mathcal{G}_b^{\text{B}} : rt \in \mathcal{R}_g^{\text{type}}} S_{r,g,t}^{\text{up}}, \qquad \forall (r,b,t) : b \in \mathcal{B} \wedge g \in \mathcal{G}_b^{\text{B}} \wedge rt \in \mathcal{R}_g^{\text{type}} \wedge t \in \mathcal{T}$$

$$\sum_{g \in \mathcal{G}_b^{\text{B}} : r \in \mathcal{R}_g^{\text{type}}} S_{r,g,t}^{\text{down}}, \qquad \forall (r,b,t) : b \in \mathcal{B} \wedge g \in \mathcal{G}_b^{\text{B}} \wedge r \in \mathcal{R}_g^{\text{type}} \wedge t \in \mathcal{T}$$

are added to the pools of available up and down spinning reserves, $\mathcal{S}^{\text{u,res}}$ and $\mathcal{S}^{\text{d,res}}$, respectively.

This module includes the same example rules ("3+5" or "Hawaii") as `balancing.operating_reserves.spinning_reserves`. These use the same formulation as described in that module, except that reserve requirements for renewable and load forecast errors are registered in $\mathcal{S}^{\text{u,req}}$ with reserve type $r^{\text{reg}}$. The Hawaii rule in this module also registers loss-of-load as a down-contingency in $\mathcal{S}^{\text{d,cont}}$ rather than a down-reserve requirement in $\mathcal{S}^{\text{d,req}}$.

This module uses the same contingency calculation options as `balancing.operating_reserves.spinning_reserves`, with identical formulations for the single-unit or entire-generation-project contingencies.

However, this module differs from `balancing.operating_reserves.spinning_reserves` in that it considers both “up” and “down” contingency requirements. It also assigns reserve type $r^{\text{cont}}$ when registering the largest contingency in each balancing area as a reserve requirement in $\mathcal{S}^{\text{u,req}}$ and $\mathcal{S}^{\text{d,req}}$.

Finally, constraints are defined to satisfy the up and down requirements for all types of spinning reserves:

$$\sum_{\left\{\substack{s^{\text{u,res}} \in \mathcal{S}^{\text{u,res}}: \\ (r,b,t) \in \mathcal{I}(s^{\text{u,res}})}\right\}} s^{\text{u,res}}_{r,b,t} \geq \sum_{\left\{\substack{s^{\text{u,req}} \in \mathcal{S}^{\text{u,req}}: \\ (r,b,t) \in \mathcal{I}(s^{\text{u,req}})}\right\}} s^{\text{u,req}}_{r,b,t}, \qquad \forall (r,b,t) \in \bigcup_{s^{\text{u,req}} \in \mathcal{S}^{\text{u,req}}} \mathcal{I}(s^{\text{u,req}}) \tag{83}$$

$$\sum_{\left\{\substack{s^{\text{d,res}} \in \mathcal{S}^{\text{d,res}}: \\ (r,b,t) \in \mathcal{I}(s^{\text{d,res}})}\right\}} s^{\text{d,res}}_{r,b,t} \geq \sum_{\left\{\substack{s^{\text{d,req}} \in \mathcal{S}^{\text{d,req}}: \\ (r,b,t) \in \mathcal{I}(s^{\text{d,req}})}\right\}} s^{\text{d,req}}_{r,b,t}, \qquad \forall (r,b,t) \in \bigcup_{s^{\text{d,req}} \in \mathcal{S}^{\text{d,req}}} \mathcal{I}(s^{\text{d,req}}), \tag{84}$$

where $\mathcal{I}(s)$ indicates the indexing set of component $s$.

As with the `balancing.operating_reserves.spinning_reserves` module, the $\mathcal{S}^{*,*}$ sets contain Pyomo components (expressions, variables or parameters) that are added to them at runtime by standard or custom modules. The $s^{*,*}$ variables refer to individual Pyomo components from these sets, and the $s^{*,*}_{r,b,t}$ terms refer to the element of $s^{*,*}$ with index $(r, b, t)$.

# 5 References

# References


[1] Stefan Pfenninger, Adam Hawkes, and James Keirstead. “Energy systems modeling for twenty-first century energy challenges”. In: *Renewable & Sustainable Energy Reviews* 33 (May 2014), pp. 74–86.

[2] Manuel Welsch et al. “Supporting security and adequacy in future energy systems: The need to enhance long-term energy system models to better treat issues related to variability”. In: *International Journal of Energy Research* 39.3 (Mar. 2015), pp. 377–396.

[3] Charles I Nweke et al. “Benefits of chronological optimization in capacity planning for electricity markets”. In: *2012 IEEE International Conference on Power System Technology (POWERCON)*. IEEE. 2012, pp. 1–6.

[4] Kris Poncelet et al. “Impact of the level of temporal and operational detail in energy-system planning models”. In: *Applied Energy* 162 (2016), pp. 631–643.

[5] B.S. Palmintier and M.D. Webster. “Impact of Operational Flexibility on Electricity Generation Planning With Renewable and Carbon Targets”. In: *IEEE Transactions on Sustainable Energy* 7.99 (2015), pp. 1–13.

[6] S. Wogrin et al. “A New Approach to Model Load Levels in Electric Power Systems With High Renewable Penetration”. In: *IEEE Transactions on Power Systems* 29.5 (2014), pp. 2210–2218. ISSN: 0885-8950. DOI: 10.1109/TPWRS.2014.2300697.

[7] C. De Jonghe, B. F. Hobbs, and R. Belmans. “Optimal Generation Mix With Short-Term Demand Response and Wind Penetration”. In: *IEEE Transactions on Power Systems* 27.2 (2012), pp. 830–839. ISSN: 0885-8950. DOI: 10.1109/TPWRS.2011.2174257.

[8] Paul Denholm et al. *Overgeneration from Solar Energy in California: A Field Guide to the Duck Chart*. Tech. rep. Report number NREL/TP-6A20-65023. 2015.

[9] Joshua-Benedict Rosenkranz, Carlo Brancucci Martinez-Anido, and Bri-Mathias Hodge. "Analyzing the Impact of Solar Power on Multi-hourly Thermal Generator Ramping". In: *2016 IEEE Green Technologies Conference (GreenTech)*. IEEE. 2016, pp. 153–158.

[10] Bryan Palmintier and Mort Webster. "Impact of unit commitment constraints on generation expansion planning with renewables". In: *2011 IEEE Power and Energy Society General Meeting*. IEEE. 2011, pp. 1–7.

[11] Francisco D Munoz and Jean-Paul Watson. "A scalable solution framework for stochastic transmission and generation planning problems". In: *Computational Management Science* 12.4 (2015), pp. 491–518.

[12] Mark Howells et al. "OSeMOSYS: the open source energy modeling system: an introduction to its ethos, structure and development". In: *Energy Policy* 39.10 (2011), pp. 5850–5870.

[13] Francisco D Munoz et al. "An engineering-economic approach to transmission planning under market and regulatory uncertainties: WECC case study". In: *IEEE Transactions on Power Systems* 29.1 (2014), pp. 307–317.

[14] Walter Short et al. *Regional Energy Deployment System (ReEDS)*. Tech. rep. Report number NREL/TP-6A20-46534. 2011.

[15] Richard Loulou. "ETSAP-TIAM: the TIMES integrated assessment model. part II: mathematical formulation". In: *Computational Management Science* 5.1-2 (2008), pp. 41–66.

[16] Manuel Welsch et al. "Incorporating flexibility requirements into long-term energy system models? A case study on high levels of renewable electricity penetration in Ireland". In: *Applied Energy* 135 (Dec. 2014), pp. 600–615.

[17] Daniel L Shawhan et al. "Does a detailed model of the electricity grid matter? Estimating the impacts of the Regional Greenhouse Gas Initiative". In: *Resource and Energy Economics* 36.1 (Jan. 2014), pp. 191–207.

[18] Kris Poncelet et al. "Selecting Representative Days for Capturing the Implications of Integrating Intermittent Renewables in Generation Expansion Planning Problems". In: *IEEE Transactions on Power Systems* 32.3 (2017), pp. 1936–1948.

[19] Matthias Fripp. "Switch: a planning tool for power systems with large shares of intermittent renewable energy". In: *Environmental Science & Technology* 46.11 (2012), pp. 6371–6378.

[20] James Nelson et al. "High-resolution modeling of the western North American power system demonstrates low-cost and low-carbon futures". In: *Energy Policy* 43 (2012), pp. 436–447.

[21] Ana Mileva et al. "SunShot solar power reduces costs and uncertainty in future low-carbon electricity systems". In: *Environmental Science & Technology* 47.16 (2013), pp. 9053–9060.

[22] Max Wei et al. "Deep carbon reductions in California require electrification and integration across economic sectors". In: *Environmental Research Letters* 8.1 (2013), p. 014038.

[23] Diego Ponce de Leon Barido et al. "Evidence and future scenarios of a low-carbon energy transition in Central America: a case study in Nicaragua". In: *Environmental Research Letters* 10.10 (Sept. 2015), p. 104002.

[24] Daniel L Sanchez et al. "Biomass enables the transition to a carbon-negative power system across western North America". In: *Nature Climate Change* 5.3 (Feb. 2015), pp. 230–234.

[25] Gang He et al. "SWITCH-China: A Systems Approach to Decarbonize China's Power System". In: *Environmental Science & Technology* (2016).

[26] Jean-Paul Watson, David L Woodruff, and William E Hart. "PySP: modeling and solving stochastic programs in Python". In: *Mathematical Programming Computation* 4.2 (2012), pp. 109–149.

[27] Ishan Sharan and R. Balasubramanian. "Integrated generation and transmission expansion planning including power and fuel transportation constraints". In: *Energy Policy* 43.C (2012), pp. 275–284.

[28] CG Heaps. "Long-range Energy Alternatives Planning (LEAP) system". In: *Somerville, MA, USA: Stockholm Environment Institute* (2016).

[29] Richard Loulou et al. "Documentation for the MARKAL Family of Models". In: *Energy Technology Systems Analysis Programme* (2004), pp. 65–73.

[30] Tom Brown, Jonas Hörsch, and David Schlachtberger. "PyPSA: Python for Power System Analysis". In: *arXiv.org* (July 2017). arXiv: `1707.09913`. URL: `https://arxiv.org/abs/1707.09913`.

[31] Richard P O'Neill et al. "A model and approach to the challenge posed by optimal power systems planning". In: *Mathematical Programming* 140.2 (2013), pp. 239–266.

[32] Cedric De Jonghe et al. "Determining optimal electricity technology mix with high level of wind power penetration". In: *Applied Energy* 88.6 (2011), pp. 2231–2238.

[33] A. van Stiphout, K. De Vos, and G. Deconinck. "The Impact of Operating Reserves on Investment Planning of Renewable Power Systems". In: *IEEE Transactions on Power Systems* 32.1 (2017), pp. 378–388.

[34] Aonghus Shortt and Mark O'Malley. "Quantifying the long-term impact of electric vehicles on the generation portfolio". In: *IEEE Transactions on Smart Grid* 5.1 (2014), pp. 71–83.

[35] E. Gil, I. Aravena, and R. Cardenas. "Generation Capacity Expansion Planning Under Hydro Uncertainty Using Stochastic Mixed Integer Programming and Scenario Reduction". In: *IEEE Transactions on Power Systems* 30.4 (2015), pp. 1838–1847.

[36] Elaine Hale, Brady Stoll, and Trieu Mai. *Capturing the impact of storage and other flexible technologies on electric system planning.* Tech. rep. NREL/TP-6A20-65726. 2016.

[37] Juan Alvarez Lopez, Kumaraswamy Ponnambalam, and Victor H Quintana. "Generation and transmission expansion under risk using stochastic programming". In: *IEEE Transactions on Power Systems* 22.3 (2007), pp. 1369–1378.

[38] Alan Valenzuela, Matias Negrete-Pincetic, and Daniel E. Olivares. "Long-Term Power Systems Planning with Operational Flexibility". In: *IEEE Transactions on Sustainable Energy* (2017). Under review.

[39] Ryan Wiser and Mark Bolinger. "Balancing cost and risk: the treatment of renewable energy in western utility resource plans". In: *The Electricity Journal* 19.1 (2006), pp. 48–59.

[40] Joseph F DeCarolis, Kevin Hunter, and Sarat Sreepathi. "The case for repeatable analysis with energy economy optimization models". In: *Energy Economics* 34.6 (Nov. 2012), pp. 1845–1853.

[41] Wided Medjroubi et al. "Open Data in Power Grid Modelling: New Approaches Towards Transparent Grid Models". In: *Energy Reports* 3 (Nov. 2017), pp. 14–21.

[42] acatech, German National Academy of Sciences Leopoldina, Union of the German Academies of Sciences and Humanities. "Consulting with energy scenarios: requirements for scientific policy advice". In: *acatech – National Academy of Science and Engineering* (2016).

[43] The Brattle Group, Energy and Environmental Economics Inc, Berkeley Economic Advising and Research LLC, Aspen Environmental Group. *Senate Bill 350 Study: The Impacts of a Regional ISO-Operated Power Market on California*. Tech. rep. 2016.

[44] California Public Utilities Commission. *Integrated Resource Plan and Long Term Procurement Plan (IRP-LTPP)*. 2017. URL: http://www.cpuc.ca.gov/irp/ (visited on 08/07/2017).

[45] HECO. *Hawaiian Electric Companies' PSIPs Update Report, Vol. 1.* Tech. rep. Available from https://www.hawaiianelectric.com/about-us/our-vision. Honolulu, Hawaii, Dec. 2016.

[46] Greg Wilson et al. "Best Practices for Scientific Computing". In: *PLOS Biology* 12.1 (Jan. 2014).
